# Supplementary material for: Spectroscopic properties of nuclear Skyrme energy density functionals
Source: arXiv:1405.4823 source file (2014-11-27)
Supplement: Supplementary file 1 [file pvc-supp-13.pdf]

# Supplemental material for: Spectroscopic properties of Skyrme energy density functionals

D. Tarpanov,[1,2] J. Dobaczewski,[1,3] J. Toivanen,[3] and B.G. Carlsson,[4]

[1]*Institute of Theoretical Physics, Faculty of Physics, University of Warsaw, Hoża 69, PL-00-681 Warsaw, Poland*
[2]*Institute for Nuclear Research and Nuclear Energy, 1784 Sofia, Bulgaria*
[3]*Department of Physics, P.O. Box 35 (YFL), University of Jyväskylä, FI-40014 Jyväskylä, Finland*
[4]*Division of Mathematical Physics, LTH, Lund University, Post Office Box 118, S-22100 Lund, Sweden*

November 13, 2014

## 1 Remarks

1. Tables 1 and 2 contain empirical and calculated data for neutrons, and Tables 3 and 4 contain empirical and calculated data for protons.
2. The Excel file, which is also provided in the supplemental material, contains all data tabulated in numerical form. It also contains results obtained for the SKX and SKXce interactions of Brown [1].
3. Figures 1, 2, 3, 4, and 5 are similar to Fig. 3 of the paper, but plotted with respect to data sets A, B, C, M, and S, respectively.
4. Figures 6, 7, 8, 9, and 10 are similar to Fig. 4 of the paper, but plotted with respect to data sets A, B, C, M, and S, respectively.
5. Figure 11 is similar to Fig. 5 of the paper.

6. Apart from the five Skyrme EDFs studied in the paper, Figs. 6–11 also show results obtained for the SKXce parametrization. This parametrization has been specifically adjusted to empirical SPEs, and indeed it describes these particular observables slightly better. Since it contains a different version of the spin-orbit interaction, it is not directly comparable to the five Skyrme EDFs presented in the paper; therefore, it is included only in this supplemental material. However, a better description of SPEs, which is obtained for the SKXce parametrization, supports the main conclusion of the paper. Indeed, the improvement of results is here obtained already at the level of bare SPEs, and not by including the PVC corrections.

   Results obtained for the SKX parametrization are almost identical to those obtained for the SKXce parametrization (see the Excel file) and thus are not included in the figures.

7. In Figs. 12–35, we plotted calculated SPEs, obtained in the present study, in comparison with those corresponding (i) to empirical data set A [2, 3, 4] and (ii) to raw experimental energies [5] measured in 24 odd nuclei, that is, in six doubly magic nuclei plus or minus one nucleon. Calculated SPEs are shown for the case of the Skyrme EDF parametrization SIII [6], for which the overall improvement brought by the PVC corrections is the largest, see Fig. 11. All energies are shown with respect to the ground-state energy of the given nucleus. For each nucleus, are shown all experimental energies measured within the energy window of the given figure. To guide the eye, we have split the experimental energies into two columns: the left column contains states connected by dashed lines to those states of the empirical data set A that have identical spins and parities, whereas the right column contains all the remaining states. This separation is provided for illustration purposes only. True association between empirical and experimental SPEs [2, 3, 4] is based on particle-transfer data, whenever they are available. For $^{55}$Ni, $^{131}$In, $^{133}$Sb, and $^{131,133}$Sn, where there is no particle-transfer data available yet, the association is based on shell-model analysis.

   We stress that the SPEs obtained after fit, which are shown in Figs. 12–35, were obtained not with the true adjustment of parameters, but within the linear approximation of the regression analysis. In addition, the fit was taking into account only the SPEs and no other observables. Therefore, results shown in Figs. 12–35 illustrate the *maximum* improvement of SPEs that one can possibly obtain within the parameter space of

the standard Skyrme functionals.

Figs. 12–35 provide us with an extensive graphic illustration of the main points discussed in the paper. First, one sees that the overall agreement of bare or PVC-corrected SPEs with empirical or experimental data is quite poor. The bare and PVC-corrected SPEs obtained after fit (a.f.) agree better with data; nevertheless the obtained level of agreement is still unsatisfactory. The figures also nicely illustrate the difficulty of extracting empirical SPEs from raw experimental energies. On the one hand, energies of low-lying single-particle states are most often quite isolated and can be quite safely associated with empirical SPEs. On the other hand, many empirical SPES are embedded within dense spectra, and are most often very strongly fragmented. However, results presented in the figures vividly show that the pattern of agreement/disagreement between calculated and empirical SPEs does not seem to be related to the excitation energy or degree of fragmentation.

One should bear in mind that results presented in Figs. 12–35 pertain to a global analysis and a global fit. Therefore, by looking at the results obtained for a single nucleus only, one should not draw too strong conclusions. Of course, the pattern of agreement/disagreement obtained in function of mass, isospin, angular momentum, etc. will be a basis of future attempts to adjust novel functionals to data.

## References


[1] A.B. Brown, Phys. Rev. C **58**, 220 (1998).

[2] H. Grawe, K. Langanke, and G. Martìnez-Pinedo, Rep. Prog. Phys. **70**, 1525 (2007).

[3] T. Faestermann, M. Górska, and H. Grawe. *Progr. in Part. Nucl. Phys.*, 69:85, 2013.

[4] H. Grawe, private communication.

[5] Evaluated Nuclear Structure Data File, http://www.nndc.bnl.gov/ensdf/.

[6] M. Beiner, H. Flocard, N. Van Giai, and P. Quentin, Nucl. Phys. **A238**, 29 (1975).

Table 1: Neutron data for $^{16}$O, $^{40}$Ca, $^{48}$Ca, and $^{56}$Ni

| level | empirical data | | | bare SPE | | | | | PVC-corrected SPE | | | | | PVC correction | | | | |
|---|---|---|---|---|---|---|---|---|---|---|---|---|---|---|---|---|---|---|
| | set A | set B | set C | SAMi | SLy5 | SIII | SkM* | SkP | SAMi | SLy5 | SIII | SkM* | SkP | SAMi | SLy5 | SIII | SkM* | SkP |
| $^{16}$O | | | | | | | | | | | | | | | | | | |
| $1p_{3/2}$ | -21.84 | | -18.60 | -20.93 | -20.61 | -20.59 | -19.89 | -18.28 | -20.94 | -20.71 | -20.69 | -19.96 | -18.46 | -0.01 | -0.10 | -0.10 | -0.07 | -0.18 |
| $1p_{1/2}$ | -15.66 | -15.66 | -12.40 | -15.50 | -14.43 | -14.54 | -13.55 | -13.61 | -16.03 | -14.73 | -15.09 | -14.29 | -14.25 | -0.53 | -0.30 | -0.55 | -0.74 | -0.64 |
| $1d_{5/2}$ | -4.14 | -4.14 | -4.14 | -6.21 | -6.82 | -6.87 | -7.30 | -7.31 | -6.33 | -7.02 | -7.00 | -7.47 | -7.57 | -0.12 | -0.20 | -0.13 | -0.17 | -0.26 |
| $2s_{1/2}$ | -3.27 | -3.27 | -3.27 | -3.34 | -3.79 | -2.77 | -4.22 | -5.35 | -4.51 | -5.12 | -4.01 | -5.78 | -6.81 | -1.17 | -1.33 | -1.24 | -1.56 | -1.46 |
| $1d_{3/2}$ | 0.94 | 1.71 | 0.94 | 0.28 | 0.50 | 0.98 | 0.41 | -1.28 | -0.07 | 0.05 | 0.67 | -0.17 | -1.92 | -0.35 | -0.45 | -0.31 | -0.58 | -0.64 |
| $^{40}$Ca | | | | | | | | | | | | | | | | | | |
| $1d_{5/2}$ | -21.27 | -22.39 | | -22.14 | -22.09 | -21.87 | -21.37 | -19.73 | -22.02 | -21.99 | -21.78 | -21.26 | -19.70 | 0.12 | 0.10 | 0.09 | 0.11 | 0.03 |
| $2s_{1/2}$ | -18.11 | -18.19 | -16.70 | -17.32 | -17.26 | -15.93 | -16.74 | -16.38 | -18.09 | -17.90 | -17.19 | -17.65 | -16.97 | -0.77 | -0.64 | -1.26 | -0.91 | -0.59 |
| $1d_{3/2}$ | -15.64 | -15.64 | -14.10 | -16.23 | -15.19 | -15.52 | -14.33 | -14.44 | -16.39 | -15.29 | -15.71 | -14.60 | -14.65 | -0.16 | -0.10 | -0.19 | -0.27 | -0.21 |
| $1f_{7/2}$ | -8.36 | -8.36 | -8.36 | -9.01 | -9.68 | -9.92 | -10.10 | -9.95 | -9.11 | -9.79 | -10.02 | -10.22 | -10.15 | -0.10 | -0.11 | -0.10 | -0.12 | -0.20 |
| $2p_{3/2}$ | -6.42 | -5.84 | -5.86 | -4.65 | -5.28 | -4.05 | -5.76 | -6.86 | -5.49 | -6.16 | -5.15 | -6.77 | -7.74 | -0.84 | -0.88 | -1.10 | -1.01 | -0.88 |
| $2p_{1/2}$ | -4.42 | -4.20 | -4.40 | -2.80 | -3.03 | -2.14 | -3.38 | -4.89 | -4.19 | -4.60 | -3.58 | -5.11 | -6.81 | -1.39 | -1.57 | -1.44 | -1.73 | -1.92 |
| $1f_{5/2}$ | -2.65 | -1.56 | -1.38 | -1.69 | -1.25 | -1.45 | -1.33 | -3.18 | -2.02 | -1.65 | -1.79 | -1.82 | -3.70 | -0.33 | -0.40 | -0.34 | -0.49 | -0.52 |
| $^{48}$Ca | | | | | | | | | | | | | | | | | | |
| $1d_{5/2}$ | | -15.61 | | -23.14 | -22.16 | -21.57 | -21.38 | -18.08 | -22.51 | -22.03 | -20.87 | -20.62 | -17.52 | 0.63 | 0.13 | 0.70 | 0.76 | 0.56 |
| $2s_{1/2}$ | | -12.55 | -12.54 | -18.48 | -17.70 | -16.37 | -17.00 | -15.67 | -17.64 | -16.13 | -16.12 | -15.75 | -15.33 | 0.84 | 1.57 | 0.25 | 1.25 | 0.34 |
| $1d_{3/2}$ | | -12.53 | -12.52 | -17.92 | -17.43 | -16.06 | -14.93 | -13.87 | -17.32 | -16.96 | -15.55 | -14.52 | -13.59 | 0.60 | 0.47 | 0.51 | 0.41 | 0.28 |
| $1f_{7/2}$ | -9.95 | -10.00 | -9.94 | -9.93 | -9.26 | -9.98 | -10.42 | -8.85 | -9.85 | -9.18 | -9.94 | -10.40 | -8.84 | 0.08 | 0.08 | 0.04 | 0.02 | 0.01 |
| $2p_{3/2}$ | -5.15 | -4.60 | -4.60 | -5.97 | -5.51 | -4.99 | -6.57 | -6.90 | -6.54 | -5.99 | -5.46 | -7.13 | -7.37 | -0.57 | -0.48 | -0.47 | -0.56 | -0.47 |
| $2p_{1/2}$ | -3.12 | -2.86 | -2.86 | -4.20 | -3.78 | -3.15 | -4.41 | -5.36 | -5.55 | -4.81 | -4.04 | -5.74 | -6.48 | -1.35 | -1.03 | -0.89 | -1.33 | -1.12 |
| $1f_{5/2}$ | -1.20 | -1.20 | -1.20 | -2.63 | -2.19 | -1.62 | -1.35 | -2.73 | -2.83 | -2.46 | -1.82 | -1.66 | -2.96 | -0.20 | -0.27 | -0.20 | -0.31 | -0.23 |
| $1g_{9/2}$ | 0.45 | 0.13 | | 2.27 | 2.61 | 1.44 | 0.37 | 0.71 | 2.08 | 2.37 | 1.26 | 0.14 | 0.44 | -0.19 | -0.24 | -0.18 | -0.23 | -0.27 |
| $^{56}$Ni | | | | | | | | | | | | | | | | | | |
| $2s_{1/2}$ | -20.40 | | -17.80 | -23.66 | -23.34 | -22.17 | -22.34 | -21.48 | -21.08 | -21.46 | -20.80 | -20.91 | -20.25 | 2.58 | 1.88 | 1.37 | 1.43 | 1.23 |
| $1d_{3/2}$ | -19.84 | | -18.40 | -24.31 | -23.54 | -22.83 | -21.57 | -20.02 | -23.35 | -22.72 | -22.08 | -20.91 | -19.32 | 0.96 | 0.82 | 0.75 | 0.66 | 0.70 |
| $1f_{7/2}$ | -16.65 | -16.64 | -14.60 | -15.81 | -16.01 | -16.11 | -16.27 | -15.45 | -15.68 | -15.91 | -16.07 | -16.23 | -15.43 | 0.13 | 0.10 | 0.04 | 0.04 | 0.02 |
| $2p_{3/2}$ | -10.25 | -10.25 | -10.25 | -10.77 | -11.10 | -10.29 | -11.36 | -12.42 | -11.56 | -11.77 | -10.92 | -12.03 | -13.25 | -0.79 | -0.67 | -0.63 | -0.67 | -0.83 |
| $1f_{5/2}$ | -9.48 | -9.48 | -9.48 | -8.61 | -8.05 | -8.22 | -7.23 | -8.46 | -9.24 | -8.63 | -8.66 | -7.81 | -8.98 | -0.63 | -0.58 | -0.44 | -0.58 | -0.52 |
| $2p_{1/2}$ | -9.14 | -9.13 | -9.14 | -9.08 | -9.21 | -8.49 | -9.36 | -10.80 | -11.37 | -10.94 | -9.96 | -11.05 | -12.21 | -2.29 | -1.73 | -1.47 | -1.69 | -1.41 |
| $1g_{9/2}$ | -6.55 | | -7.24 | -3.32 | -4.02 | -4.53 | -5.16 | -5.78 | -3.88 | -4.51 | -4.97 | -5.57 | -6.38 | -0.56 | -0.49 | -0.44 | -0.41 | -0.60 |

Table 2: Neutron data for $^{132}$Sn and $^{208}$Pb

| level | empirical data | | | bare SPE | | | | | PVC-corrected SPE | | | | | PVC correction | | | | |
|---|---|---|---|---|---|---|---|---|---|---|---|---|---|---|---|---|---|---|
| | set A | set B | set C | SAMi | SLY5 | SIII | SkM* | SkP | SAMi | SLY5 | SIII | SkM* | SkP | SAMi | SLY5 | SIII | SkM* | SkP |
| $^{132}$Sn | | | | | | | | | | | | | | | | | | |
| $1g_{7/2}$ | -9.82 | -9.75 | -9.75 | -13.16 | -11.67 | -11.25 | -10.15 | -8.81 | -12.82 | -11.36 | -10.97 | -9.90 | -8.60 | 0.34 | 0.31 | 0.28 | 0.25 | 0.21 |
| $2d_{5/2}$ | -9.04 | -8.97 | -8.97 | -12.51 | -11.79 | -10.70 | -11.48 | -10.47 | -11.77 | -11.08 | -10.29 | -11.04 | -10.09 | 0.74 | 0.71 | 0.41 | 0.44 | 0.38 |
| $3s_{1/2}$ | -7.72 | -7.64 | -7.64 | -10.17 | -9.54 | -8.32 | -9.29 | -8.89 | -9.33 | -8.64 | -7.71 | -8.74 | -8.39 | 0.84 | 0.90 | 0.61 | 0.55 | 0.50 |
| $1h_{11/2}$ | -7.63 | -7.54 | -7.38 | -8.19 | -7.47 | -8.16 | -8.47 | -7.00 | -8.11 | -7.39 | -8.10 | -8.42 | -6.97 | 0.08 | 0.08 | 0.06 | 0.05 | 0.03 |
| $2d_{3/2}$ | -7.39 | -7.31 | -7.31 | -10.28 | -9.23 | -8.24 | -8.84 | -8.46 | -9.95 | -8.87 | -7.99 | -8.62 | -8.25 | 0.33 | 0.36 | 0.25 | 0.22 | 0.21 |
| $2f_{7/2}$ | -2.45 | -2.47 | -2.47 | -2.62 | -2.08 | -1.73 | -3.13 | -3.39 | -2.79 | -2.22 | -1.87 | -3.29 | -3.52 | -0.17 | -0.14 | -0.14 | -0.16 | -0.13 |
| $3p_{3/2}$ | -1.59 | -1.57 | -1.62 | -0.76 | -0.01 | 0.22 | -1.17 | -1.67 | -1.25 | -0.36 | -0.13 | -1.71 | -2.17 | -0.49 | -0.35 | -0.35 | -0.54 | -0.50 |
| $1h_{9/2}$ | -0.88 | -0.86 | -0.91 | -0.92 | 0.54 | 0.05 | 0.68 | 0.04 | -1.02 | 0.44 | -0.03 | 0.56 | -0.05 | -0.10 | -0.10 | -0.08 | -0.12 | -0.09 |
| $3p_{1/2}$ | -0.79 | | | -0.18 | 0.71 | 0.88 | -0.40 | -0.98 | -0.96 | 0.21 | 0.42 | -1.28 | -1.78 | -0.78 | -0.50 | -0.46 | -0.88 | -0.80 |
| $2f_{5/2}$ | -0.44 | -0.42 | -0.47 | -0.27 | 0.67 | 0.92 | -0.18 | -0.96 | -0.56 | 0.44 | 0.72 | -0.47 | -1.20 | -0.29 | -0.23 | -0.20 | -0.29 | -0.24 |
| $1i_{13/2}$ | 0.25 | | | 1.99 | 2.52 | 1.09 | 0.30 | 0.67 | 1.78 | 2.32 | 0.95 | 0.15 | 0.52 | -0.21 | -0.20 | -0.14 | -0.15 | -0.15 |
| $^{208}$Pb | | | | | | | | | | | | | | | | | | |
| $1h_{9/2}$ | -10.78 | -11.40 | -10.78 | -14.18 | -12.73 | -12.56 | -11.39 | -10.13 | -13.96 | -12.53 | -12.37 | -11.24 | -10.01 | 0.22 | 0.20 | 0.19 | 0.15 | 0.12 |
| $2f_{7/2}$ | -9.71 | -9.81 | -10.30 | -12.81 | -12.08 | -11.25 | -11.92 | -10.94 | -12.28 | -11.59 | -10.91 | -11.62 | -10.68 | 0.53 | 0.49 | 0.34 | 0.30 | 0.26 |
| $1i_{13/2}$ | -9.00 | -9.24 | -9.80 | -10.05 | -9.37 | -10.12 | -10.21 | -8.78 | -9.98 | -9.30 | -10.06 | -10.17 | -8.77 | 0.07 | 0.07 | 0.06 | 0.04 | 0.01 |
| $3p_{3/2}$ | -8.27 | -8.26 | -8.27 | -9.89 | -9.31 | -8.24 | -9.26 | -8.92 | -9.62 | -9.02 | -8.05 | -9.10 | -8.76 | 0.27 | 0.29 | 0.19 | 0.16 | 0.16 |
| $2f_{5/2}$ | -7.94 | -7.94 | -7.94 | -10.28 | -9.14 | -8.47 | -8.91 | -8.65 | -10.11 | -8.96 | -8.35 | -8.79 | -8.52 | 0.17 | 0.18 | 0.12 | 0.12 | 0.13 |
| $3p_{1/2}$ | -7.37 | -7.37 | -7.37 | -8.94 | -8.21 | -7.21 | -8.14 | -8.10 | -8.72 | -7.88 | -7.10 | -8.12 | -7.99 | 0.22 | 0.33 | 0.11 | 0.02 | 0.11 |
| $2g_{9/2}$ | -3.94 | -3.94 | -3.94 | -3.72 | -3.25 | -3.01 | -4.24 | -4.46 | -3.85 | -3.36 | -3.16 | -4.37 | -4.57 | -0.13 | -0.11 | -0.15 | -0.13 | -0.11 |
| $1i_{11/2}$ | -3.16 | -3.16 | -3.16 | -3.33 | -1.88 | -2.67 | -1.76 | -2.27 | -3.37 | -1.93 | -2.71 | -1.83 | -2.34 | -0.04 | -0.05 | -0.04 | -0.07 | -0.07 |
| $1j_{15/2}$ | -2.51 | -2.51 | -2.52 | -0.84 | -0.34 | -1.85 | -2.32 | -1.94 | -1.01 | -0.51 | -1.99 | -2.45 | -2.07 | -0.17 | -0.17 | -0.14 | -0.13 | -0.13 |
| $3d_{5/2}$ | -2.37 | -2.37 | -2.37 | -1.11 | -0.57 | -0.24 | -1.67 | -2.32 | -1.44 | -0.83 | -0.55 | -2.01 | -2.59 | -0.33 | -0.26 | -0.31 | -0.34 | -0.27 |
| $4s_{1/2}$ | -1.90 | -1.90 | -1.90 | -0.28 | 0.50 | 0.64 | -0.72 | -1.34 | -1.30 | -0.25 | -0.15 | -1.85 | -2.32 | -1.02 | -0.75 | -0.79 | -1.13 | -0.98 |
| $2g_{7/2}$ | -1.45 | -1.44 | -1.44 | -0.95 | -0.01 | 0.09 | -0.83 | -1.75 | -1.13 | -0.15 | -0.07 | -1.01 | -1.90 | -0.18 | -0.14 | -0.16 | -0.18 | -0.15 |
| $3d_{3/2}$ | -1.40 | -1.40 | -1.40 | -0.12 | 0.63 | 0.86 | -0.40 | -1.26 | -0.55 | 0.33 | 0.55 | -0.84 | -1.63 | -0.43 | -0.30 | -0.31 | -0.44 | -0.37 |

Table 3: Proton data for $^{16}$O, $^{40}$Ca, $^{48}$Ca, and $^{56}$Ni

| level | empirical data | | | bare SPE | | | | | PVC-corrected SPE | | | | | PVC correction | | | | |
|---|---|---|---|---|---|---|---|---|---|---|---|---|---|---|---|---|---|---|
| | set A | set B | set C | SAMi | SLy5 | SIII | SkM* | SkP | SAMi | SLy5 | SIII | SkM* | SkP | SAMi | SLy5 | SIII | SkM* | SkP |
| $^{16}$O | | | | | | | | | | | | | | | | | | |
| $1p_{3/2}$ | -18.45 | | -15.30 | -17.44 | -17.14 | -17.09 | -16.48 | -14.93 | -17.45 | -17.22 | -17.18 | -16.50 | -15.06 | -0.01 | -0.08 | -0.09 | -0.02 | -0.13 |
| $1p_{1/2}$ | -12.13 | -12.13 | -9.00 | -12.07 | -11.08 | -11.15 | -10.27 | -10.36 | -12.58 | -11.30 | -11.68 | -10.99 | -10.94 | -0.51 | -0.22 | -0.53 | -0.72 | -0.58 |
| $1d_{5/2}$ | -0.60 | -0.60 | -0.60 | -3.00 | -3.62 | -3.59 | -4.10 | -4.12 | -3.10 | -3.80 | -3.70 | -4.23 | -4.31 | -0.10 | -0.18 | -0.11 | -0.13 | -0.19 |
| $2s_{1/2}$ | -0.11 | -0.11 | -0.10 | -0.33 | -0.77 | 0.27 | -1.20 | -2.25 | -1.38 | -1.95 | -0.82 | -2.59 | -3.52 | -1.05 | -1.18 | -1.09 | -1.39 | -1.27 |
| $1d_{3/2}$ | 4.40 | 4.69 | 4.40 | 3.23 | 3.39 | 3.93 | 3.28 | 1.68 | 2.91 | 3.01 | 3.66 | 2.77 | 1.16 | -0.32 | -0.38 | -0.27 | -0.51 | -0.52 |
| $^{40}$Ca | | | | | | | | | | | | | | | | | | |
| $1d_{5/2}$ | -13.73 | -15.07 | | -14.98 | -14.95 | -14.74 | -14.33 | -12.75 | -14.82 | -14.80 | -14.59 | -14.16 | -12.65 | 0.16 | 0.15 | 0.15 | 0.17 | 0.10 |
| $2s_{1/2}$ | -10.85 | -10.92 | -8.94 | -10.14 | -10.16 | -8.78 | -9.74 | -9.41 | -10.83 | -10.69 | -9.86 | -10.49 | -9.79 | -0.69 | -0.53 | -1.08 | -0.75 | -0.38 |
| $1d_{3/2}$ | -8.33 | -8.33 | -6.42 | -9.16 | -8.24 | -8.53 | -7.48 | -7.61 | -9.29 | -8.30 | -8.64 | -7.68 | -7.72 | -0.13 | -0.06 | -0.11 | -0.20 | -0.11 |
| $1f_{7/2}$ | -1.09 | -1.09 | -1.09 | -2.24 | -2.90 | -3.08 | -3.34 | -3.19 | -2.28 | -2.97 | -3.10 | -3.39 | -3.28 | -0.04 | -0.07 | -0.02 | -0.05 | -0.09 |
| $2p_{3/2}$ | 0.63 | 0.69 | 0.69 | 1.79 | 1.18 | 2.43 | 0.73 | -0.23 | 1.13 | 0.49 | 1.60 | -0.06 | -0.88 | -0.66 | -0.69 | -0.83 | -0.79 | -0.65 |
| $2p_{1/2}$ | 2.38 | 2.38 | 2.41 | 3.40 | 3.14 | 4.04 | 2.81 | 1.54 | 2.38 | 2.00 | 3.23 | 1.53 | 0.11 | -1.02 | -1.14 | -0.81 | -1.28 | -1.43 |
| $1f_{5/2}$ | 4.60 | 4.96 | | 4.74 | 5.07 | 5.01 | 4.96 | 3.27 | 4.48 | 4.76 | 4.79 | 4.58 | 2.90 | -0.26 | -0.31 | -0.22 | -0.38 | -0.37 |
| $^{48}$Ca | | | | | | | | | | | | | | | | | | |
| $1d_{5/2}$ | -21.58 | -21.47 | | -21.67 | -22.45 | -21.83 | -21.16 | -20.26 | -21.52 | -22.28 | -21.73 | -21.06 | -20.20 | 0.15 | 0.17 | 0.10 | 0.10 | 0.06 |
| $1d_{3/2}$ | -16.17 | -16.18 | -16.68 | -16.36 | -15.34 | -16.24 | -14.69 | -14.54 | -16.32 | -15.31 | -16.20 | -14.70 | -14.48 | 0.04 | 0.03 | 0.04 | -0.01 | 0.06 |
| $2s_{1/2}$ | -15.81 | -16.10 | -16.39 | -16.05 | -16.74 | -15.28 | -15.64 | -15.98 | -16.48 | -17.17 | -15.89 | -16.09 | -16.25 | -0.43 | -0.43 | -0.61 | -0.45 | -0.27 |
| $1f_{7/2}$ | -9.63 | -9.35 | -9.63 | -8.93 | -10.70 | -10.16 | -9.94 | -10.74 | -9.21 | -11.00 | -10.42 | -10.19 | -11.10 | -0.28 | -0.30 | -0.26 | -0.25 | -0.36 |
| $2p_{3/2}$ | -6.55 | -6.44 | | -3.25 | -4.89 | -2.99 | -4.30 | -6.27 | -3.96 | -5.65 | -3.76 | -5.12 | -7.12 | -0.71 | -0.76 | -0.77 | -0.82 | -0.85 |
| $2p_{1/2}$ | -5.05 | -4.64 | | -1.53 | -2.57 | -1.21 | -2.20 | -4.32 | -3.23 | -4.47 | -2.72 | -3.98 | -6.09 | -1.70 | -1.90 | -1.51 | -1.78 | -1.77 |
| $1f_{5/2}$ | -4.55 | | | -1.60 | -1.32 | -2.01 | -1.11 | -3.04 | -2.10 | -1.84 | -2.52 | -1.74 | -3.70 | -0.50 | -0.52 | -0.51 | -0.63 | -0.66 |
| $^{56}$Ni | | | | | | | | | | | | | | | | | | |
| $2s_{1/2}$ | -10.73 | | -7.90 | -14.06 | -13.87 | -12.66 | -12.90 | -12.18 | -11.66 | -12.07 | -11.19 | -11.42 | -10.80 | 2.40 | 1.80 | 1.47 | 1.48 | 1.38 |
| $1d_{3/2}$ | -10.09 | | -8.60 | -14.80 | -14.01 | -13.46 | -12.25 | -10.78 | -13.79 | -13.14 | -12.62 | -11.50 | -9.89 | 1.01 | 0.87 | 0.84 | 0.75 | 0.89 |
| $1f_{7/2}$ | -7.17 | -7.17 | -5.00 | -6.72 | -6.93 | -6.98 | -7.15 | -6.40 | -6.52 | -6.77 | -6.87 | -7.08 | -6.31 | 0.20 | 0.16 | 0.11 | 0.07 | 0.09 |
| $2p_{3/2}$ | -0.69 | -0.69 | -0.69 | -1.77 | -2.16 | -1.23 | -2.36 | -3.37 | -2.31 | -2.62 | -1.65 | -2.86 | -3.94 | -0.54 | -0.46 | -0.42 | -0.50 | -0.57 |
| $1f_{5/2}$ | 0.34 | 0.33 | 0.42 | 0.32 | 0.84 | 0.69 | 1.58 | 0.40 | -0.20 | 0.38 | 0.36 | 1.09 | 0.04 | -0.52 | -0.46 | -0.33 | -0.49 | -0.36 |
| $2p_{1/2}$ | 0.42 | 0.41 | 0.34 | -0.24 | -0.44 | 0.39 | -0.54 | -1.88 | -1.93 | -1.73 | -0.64 | -1.84 | -2.77 | -1.69 | -1.29 | -1.03 | -1.30 | -0.89 |
| $1g_{9/2}$ | 2.82 | | 2.82 | 5.29 | 4.63 | 4.23 | 3.59 | 3.00 | 4.86 | 4.25 | 3.90 | 3.25 | 2.54 | -0.43 | -0.38 | -0.33 | -0.34 | -0.46 |

Table 4: Proton data for $^{132}$Sn and $^{208}$Pb

| level | empirical data | | | bare SPE | | | | | PVC-corrected SPE | | | | | PVC correction | | | | |
|---|---|---|---|---|---|---|---|---|---|---|---|---|---|---|---|---|---|---|
| | set A | set B | set C | SAMi | SLy5 | SIII | SkM* | SkP | SAMi | SLy5 | SIII | SkM* | SkP | SAMi | SLy5 | SIII | SkM* | SkP |
| $^{132}$Sn | | | | | | | | | | | | | | | | | | |
| $1f_{5/2}$ | -18.36 | | | -20.32 | -20.65 | -20.48 | -18.93 | -18.32 | -19.96 | -20.36 | -20.18 | -18.69 | -18.12 | 0.36 | 0.29 | 0.30 | 0.24 | 0.20 |
| $2p_{3/2}$ | -17.14 | | | -17.87 | -18.90 | -17.84 | -17.56 | -17.83 | -17.30 | -18.49 | -17.52 | -17.24 | -17.60 | 0.57 | 0.41 | 0.32 | 0.32 | 0.23 |
| $2p_{1/2}$ | -16.13 | -16.01 | -16.01 | -16.56 | -17.44 | -16.49 | -16.11 | -16.69 | -16.43 | -17.42 | -16.45 | -16.08 | -16.67 | 0.13 | 0.02 | 0.04 | 0.03 | 0.02 |
| $1g_{9/2}$ | -15.78 | -15.71 | -15.71 | -14.11 | -15.44 | -15.29 | -14.60 | -14.69 | -14.08 | -15.42 | -15.29 | -14.60 | -14.69 | 0.03 | 0.02 | 0.00 | 0.00 | 0.00 |
| $1g_{7/2}$ | -9.65 | -9.68 | -9.68 | -8.53 | -9.23 | -9.50 | -7.90 | -9.17 | -8.70 | -9.45 | -9.69 | -8.11 | -9.39 | -0.17 | -0.22 | -0.19 | -0.21 | -0.22 |
| $2d_{5/2}$ | -8.69 | -8.72 | -8.72 | -7.44 | -9.06 | -7.92 | -8.28 | -9.88 | -7.91 | -9.55 | -8.40 | -8.72 | -10.32 | -0.47 | -0.49 | -0.48 | -0.44 | -0.44 |
| $2d_{3/2}$ | -6.95 | -6.97 | -7.24 | -5.41 | -6.79 | -5.80 | -5.98 | -8.09 | -6.29 | -7.61 | -6.60 | -6.72 | -8.76 | -0.88 | -0.82 | -0.80 | -0.74 | -0.67 |
| $1h_{11/2}$ | -6.86 | -6.89 | | -4.10 | -6.07 | -5.99 | -5.54 | -6.84 | -4.33 | -6.31 | -6.22 | -5.77 | -7.06 | -0.23 | -0.24 | -0.23 | -0.23 | -0.22 |
| $^{208}$Pb | | | | | | | | | | | | | | | | | | |
| $1g_{7/2}$ | -11.49 | -12.00 | | -13.19 | -13.49 | -13.51 | -11.93 | -11.45 | -12.93 | -13.26 | -13.27 | -11.73 | -11.29 | 0.26 | 0.23 | 0.24 | 0.20 | 0.16 |
| $2d_{5/2}$ | -9.70 | -9.82 | | -10.28 | -11.35 | -10.29 | -10.16 | -10.39 | -9.86 | -11.03 | -9.99 | -9.89 | -10.19 | 0.42 | 0.32 | 0.30 | 0.27 | 0.20 |
| $1h_{11/2}$ | -9.36 | -9.36 | -9.35 | -8.35 | -9.57 | -9.58 | -8.80 | -8.76 | -8.28 | -9.51 | -9.51 | -8.75 | -8.74 | 0.07 | 0.06 | 0.07 | 0.05 | 0.02 |
| $2d_{3/2}$ | -8.36 | -8.36 | -8.35 | -8.55 | -9.43 | -8.52 | -8.22 | -8.92 | -8.46 | -9.37 | -8.47 | -8.16 | -8.91 | 0.09 | 0.06 | 0.05 | 0.06 | 0.01 |
| $3s_{1/2}$ | -8.01 | -8.01 | -8.10 | -7.60 | -8.74 | -7.41 | -7.60 | -8.29 | -7.32 | -8.54 | -7.26 | -7.50 | -8.30 | 0.28 | 0.20 | 0.15 | 0.10 | -0.01 |
| $1h_{9/2}$ | -3.80 | -3.80 | -3.80 | -3.10 | -3.72 | -4.17 | -2.54 | -3.63 | -3.14 | -3.78 | -4.21 | -2.60 | -3.73 | -0.04 | -0.06 | -0.04 | -0.06 | -0.10 |
| $2f_{7/2}$ | -2.90 | -2.90 | -2.49 | -1.25 | -2.82 | -1.73 | -2.11 | -3.48 | -1.46 | -3.03 | -1.98 | -2.30 | -3.69 | -0.21 | -0.21 | -0.25 | -0.19 | -0.21 |
| $1i_{13/2}$ | -2.19 | -2.10 | -1.83 | 0.42 | -1.33 | -1.49 | -0.91 | -1.93 | 0.26 | -1.47 | -1.61 | -1.03 | -2.07 | -0.16 | -0.14 | -0.12 | -0.12 | -0.14 |
| $2f_{5/2}$ | -0.98 | -0.97 | -0.40 | 1.05 | -0.27 | 0.64 | 0.50 | -1.47 | 0.66 | -0.59 | 0.27 | 0.19 | -1.81 | -0.39 | -0.32 | -0.37 | -0.31 | -0.34 |
| $3p_{3/2}$ | -0.68 | -0.68 | | 2.06 | 0.47 | 1.89 | 1.04 | -0.80 | 1.25 | -0.32 | 1.06 | 0.29 | -1.58 | -0.81 | -0.79 | -0.83 | -0.75 | -0.78 |
| $3p_{1/2}$ | -0.17 | -0.16 | | 2.87 | 1.41 | 2.72 | 1.97 | -0.10 | 1.53 | 0.08 | 1.58 | 0.75 | -1.50 | -1.34 | -1.33 | -1.14 | -1.22 | -1.40 |

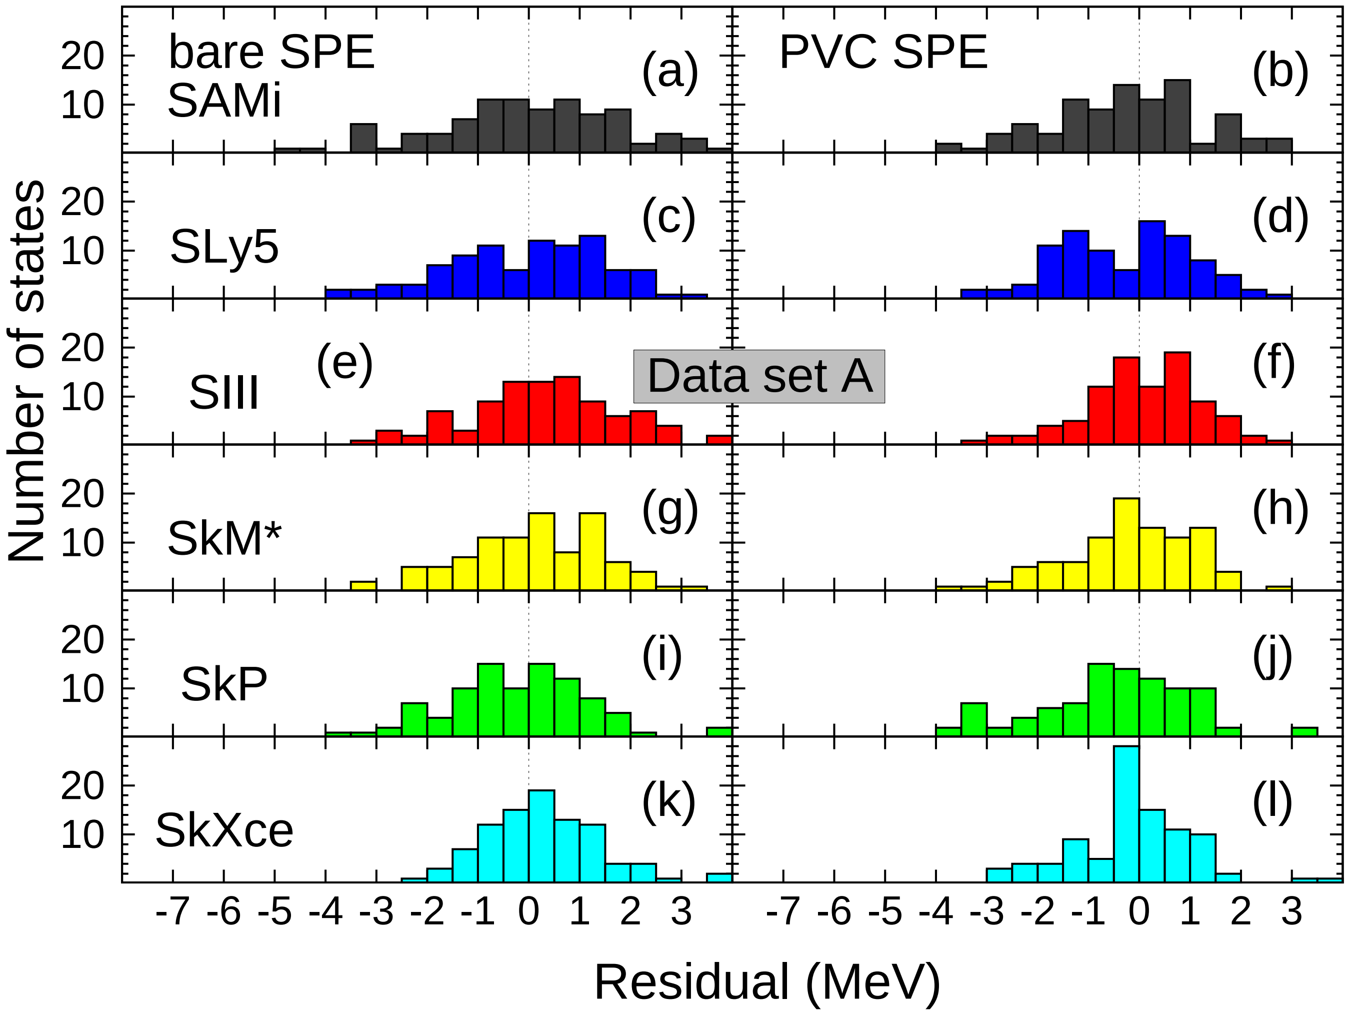


Figure 1: (Color online) Similar to Fig. 3 of the paper, but with Skyrme EDF SKXce included.

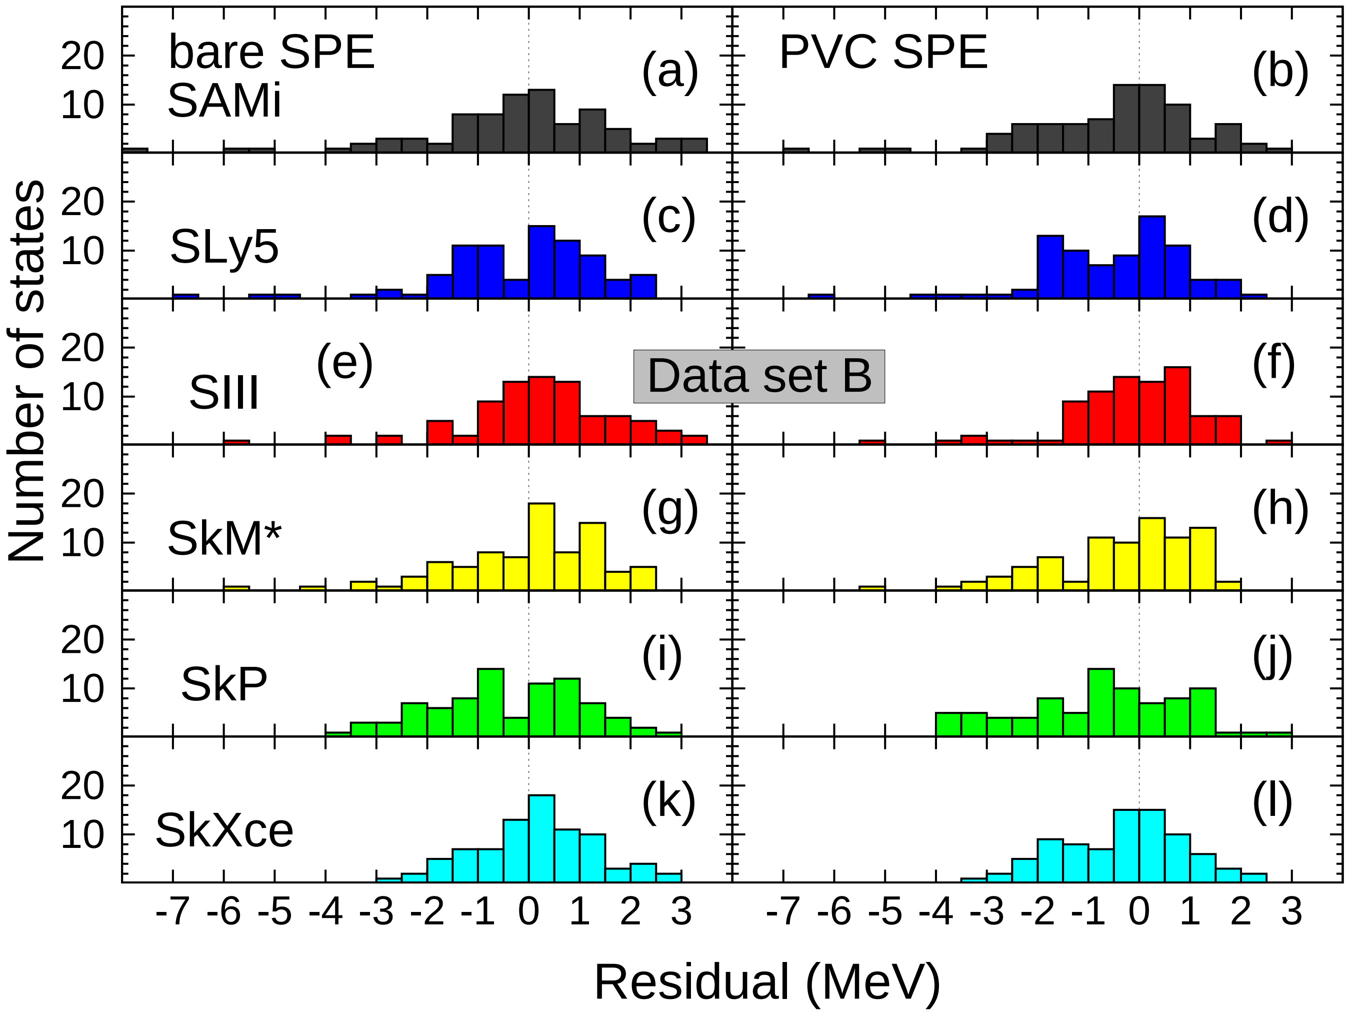


Figure 2: (Color online) Similar to Fig. 3 of the paper, but for data set B and with Skyrme EDF SKXce included.

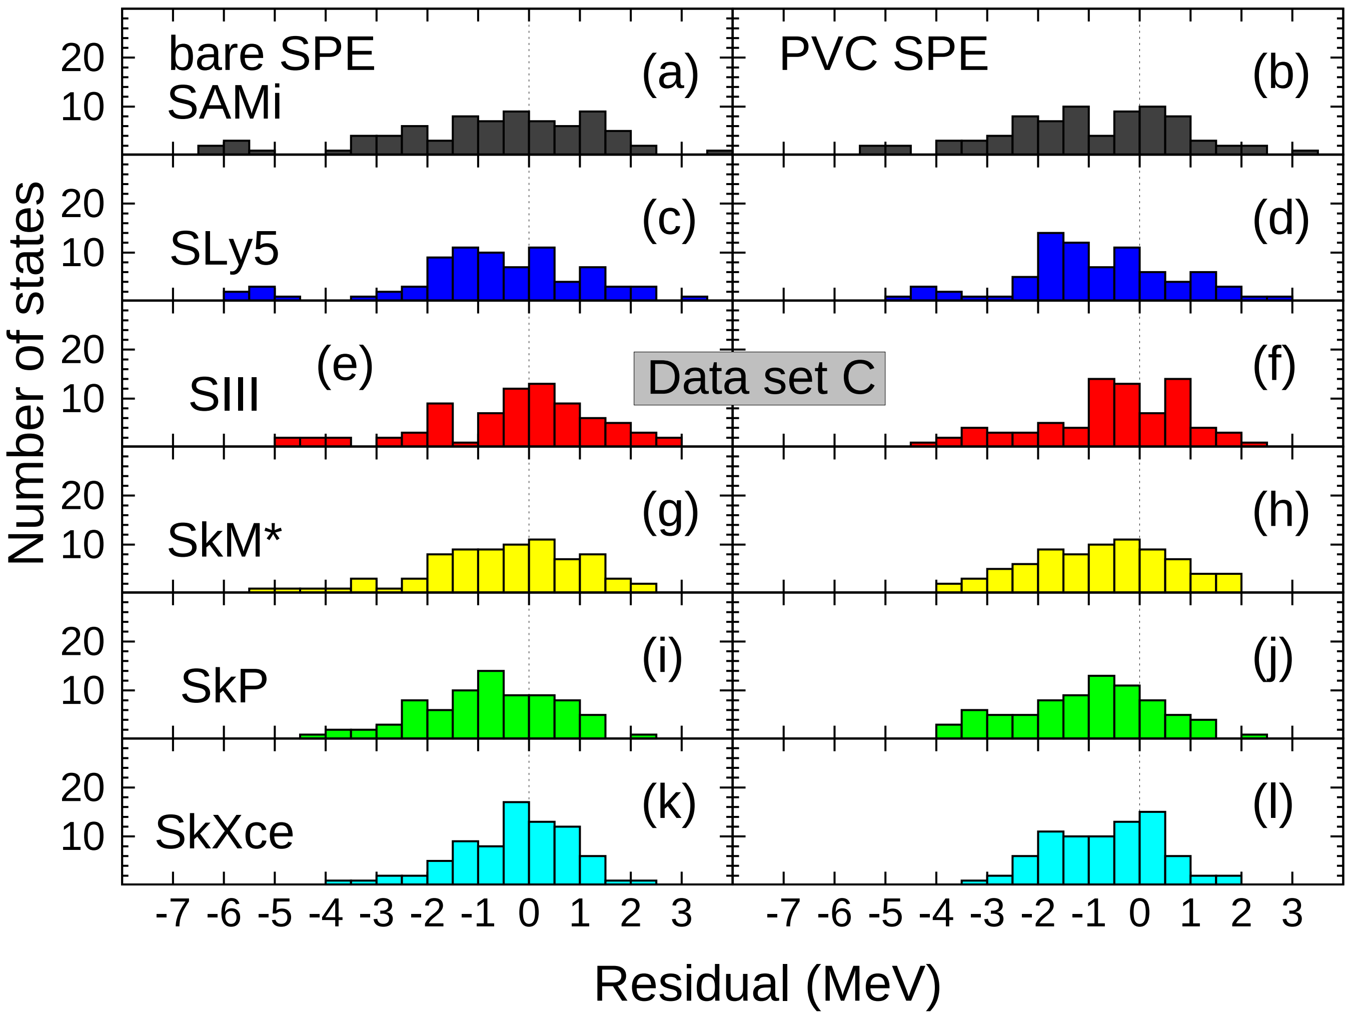


Figure 3: (Color online) Similar to Fig. 3 of the paper, but for data set C and with Skyrme EDF SKXce included.

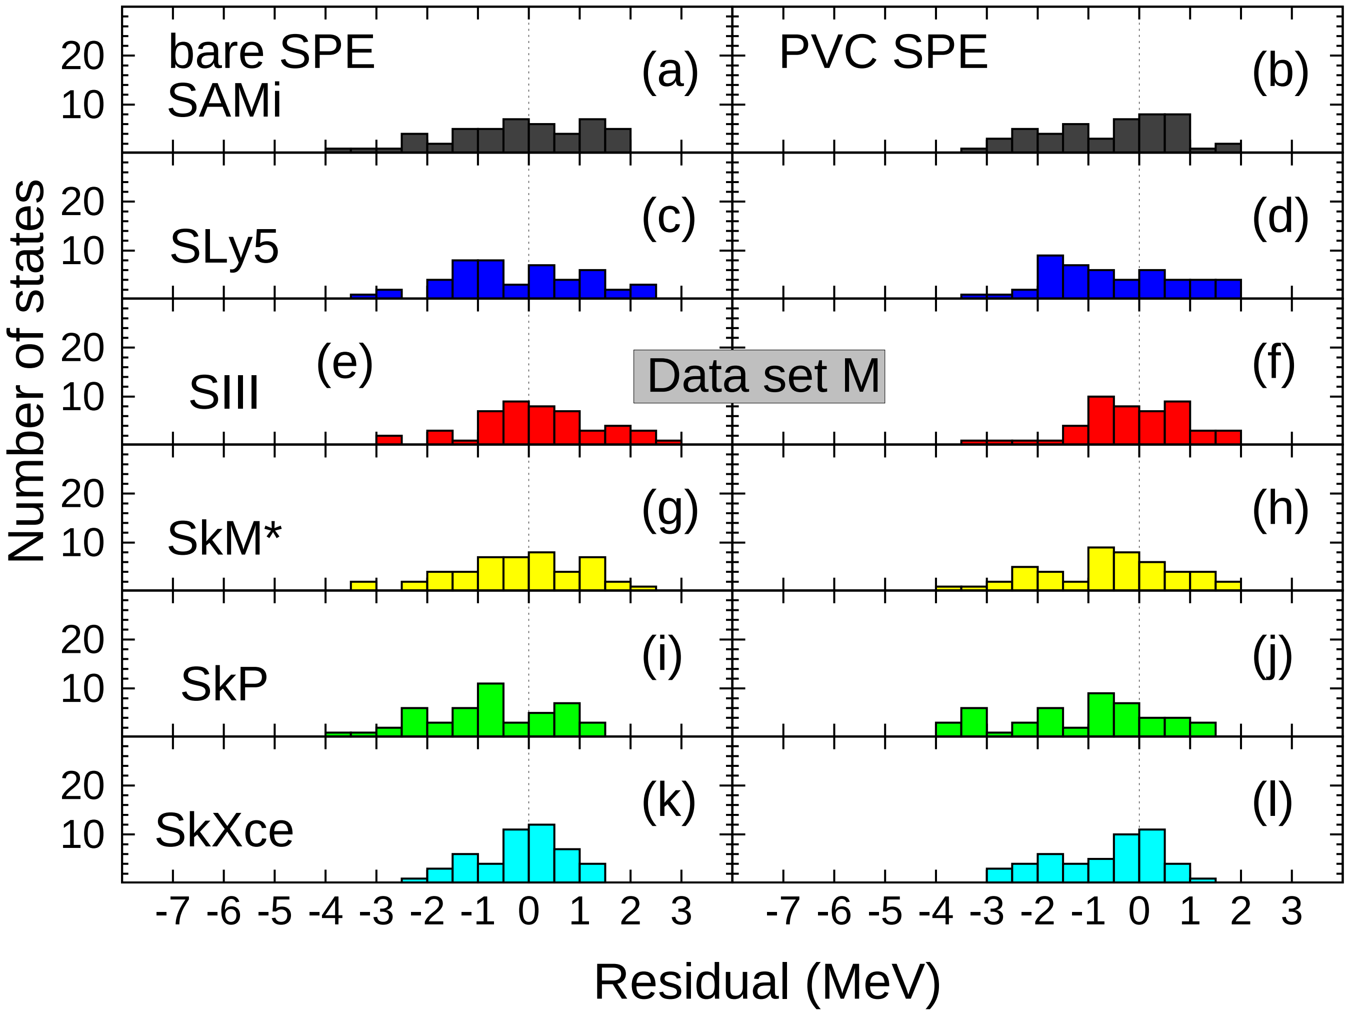


Figure 4: (Color online) Similar to Fig. 3 of the paper, but for data set M and with Skyrme EDF SKXce included.

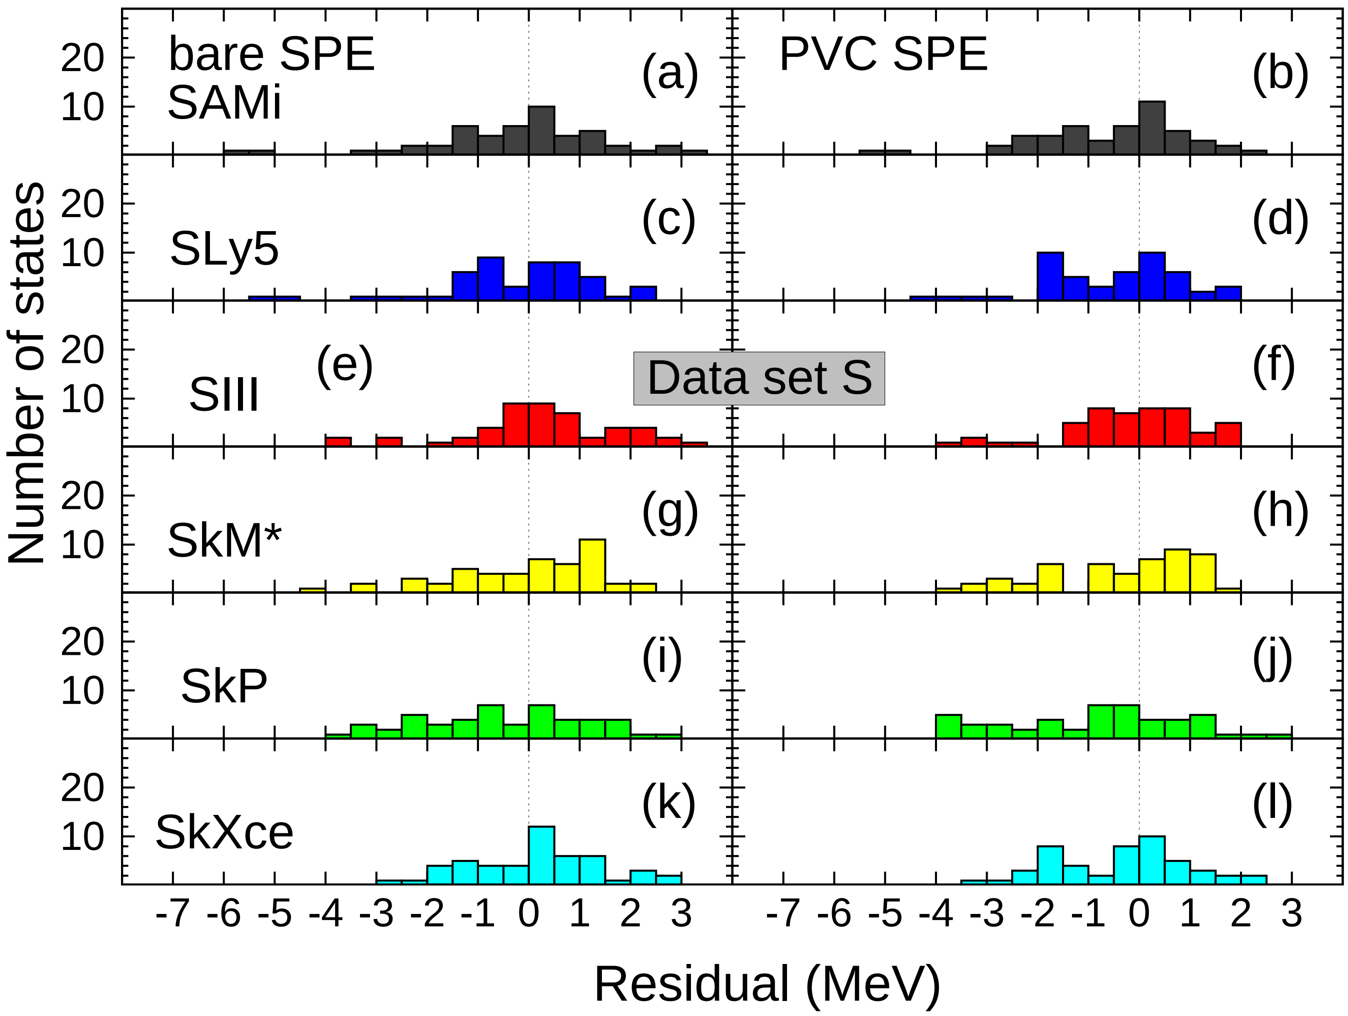


Figure 5: (Color online) Similar to Fig. 3 of the paper, but for data set S and with Skyrme EDF SKXce included.

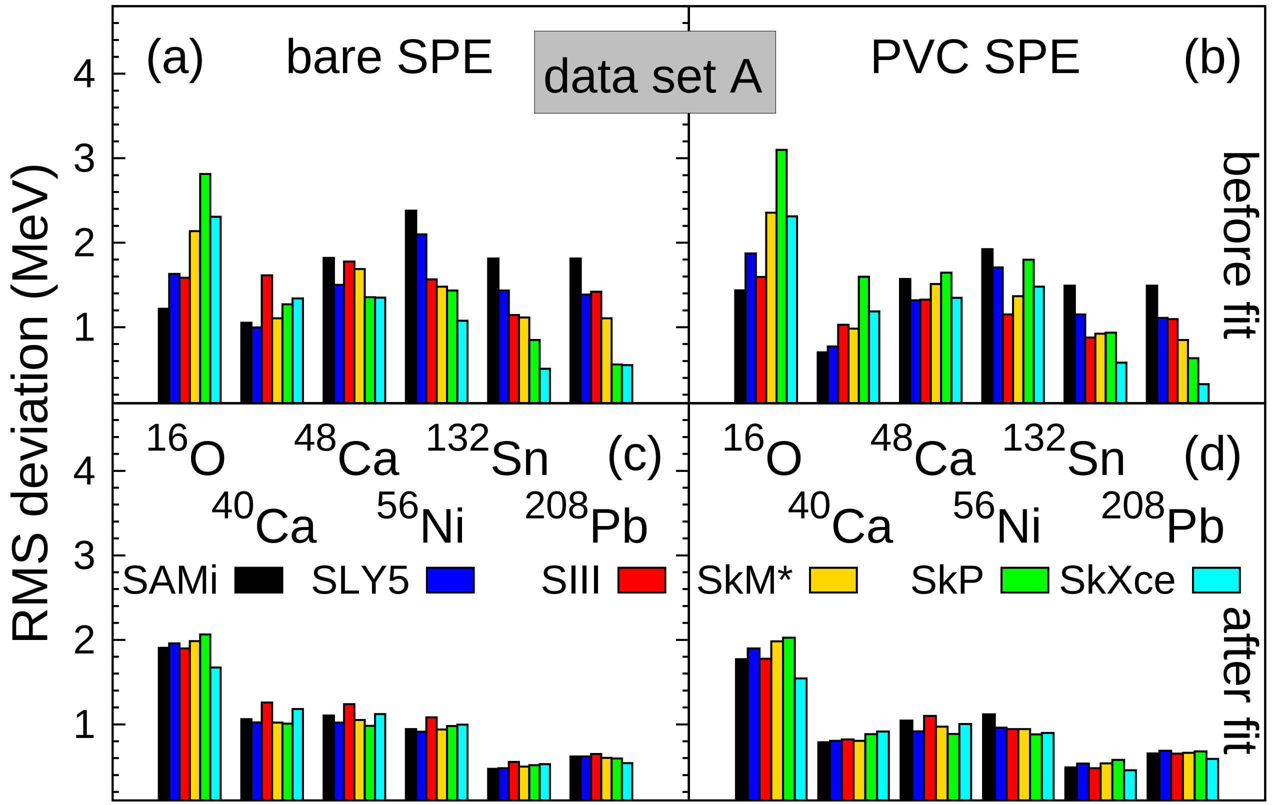


Figure 6: (Color online) Similar to Fig. 4 of the paper, but with Skyrme EDF SKXce included.

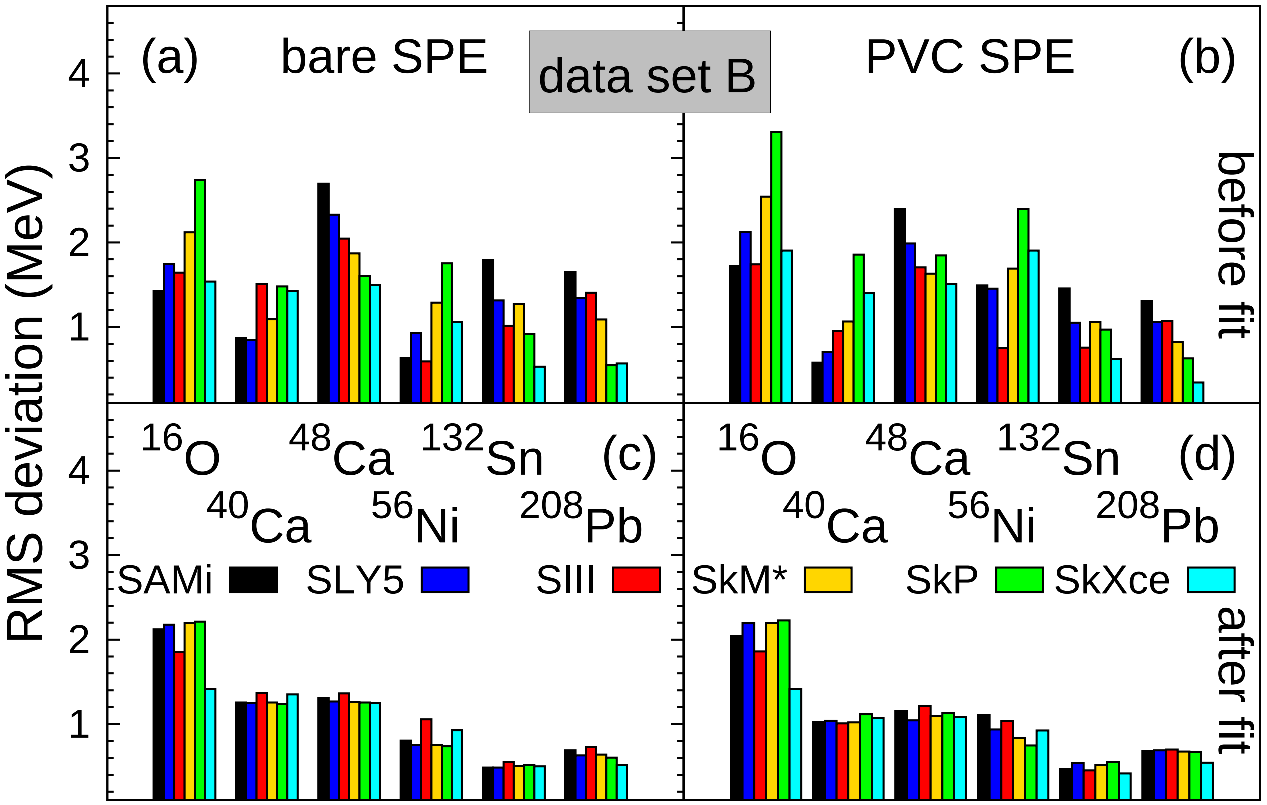


Figure 7: (Color online) Similar to Fig. 4 of the paper, but for data set B and with Skyrme EDF SKXce included.

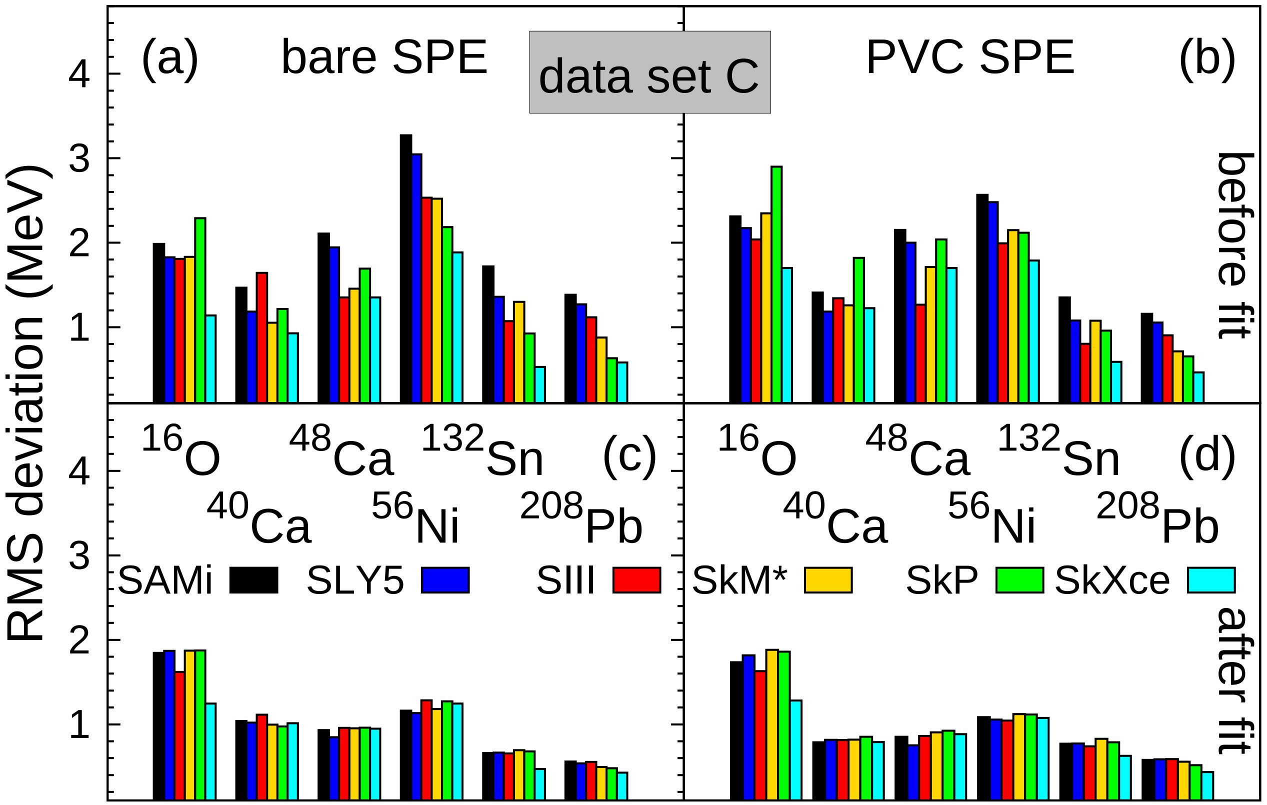


Figure 8: (Color online) Similar to Fig. 4 of the paper, but for data set C and with Skyrme EDF SKXce included.

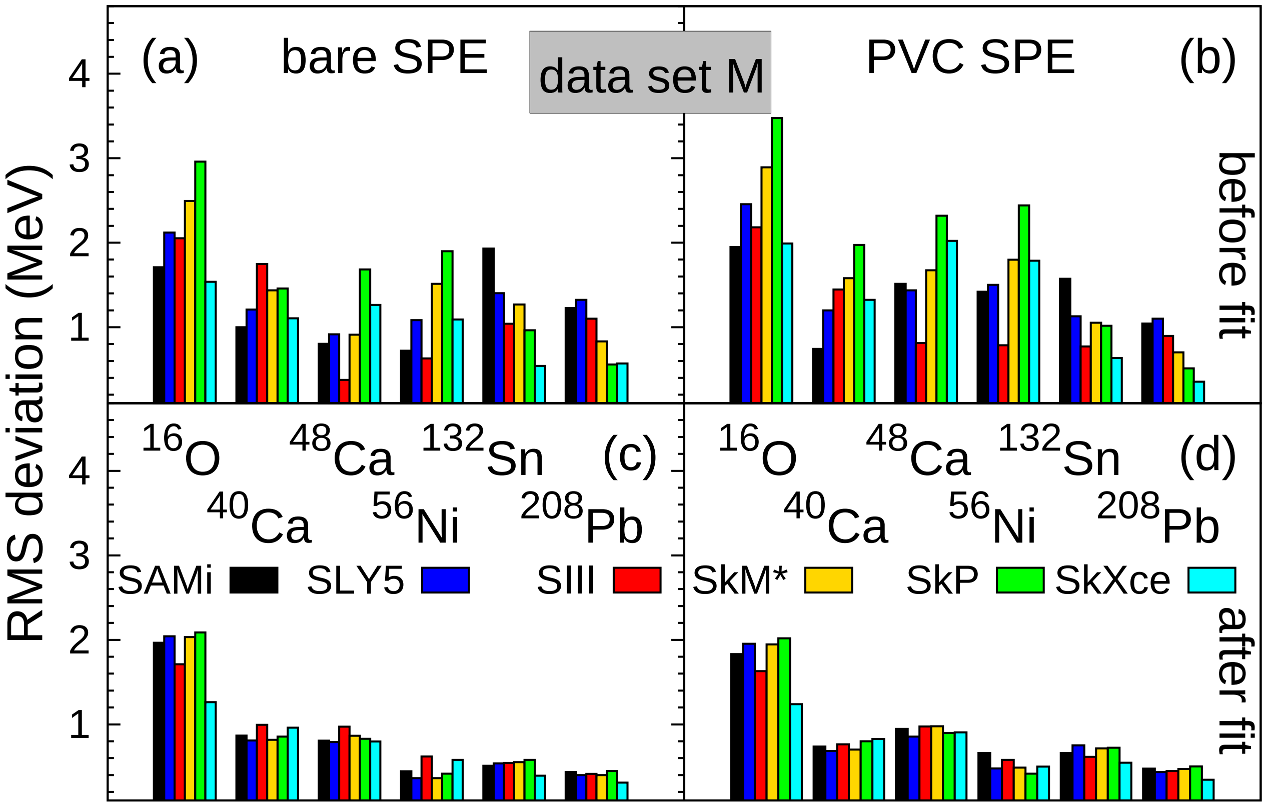


Figure 9: (Color online) Similar to Fig. 4 of the paper, but for data set M and with Skyrme EDF SKXce included.

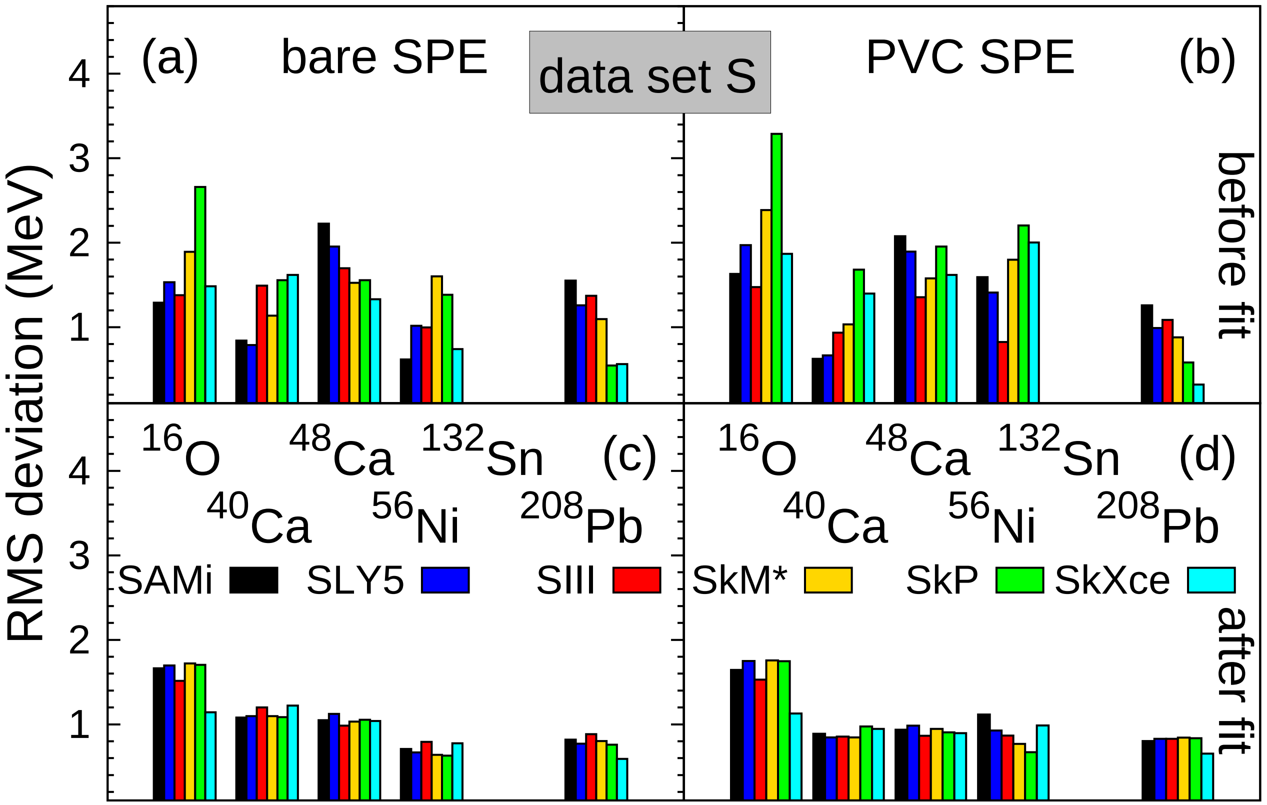


Figure 10: (Color online) Similar to Fig. 4 of the paper, but for data set S and with Skyrme EDF SKXce included.

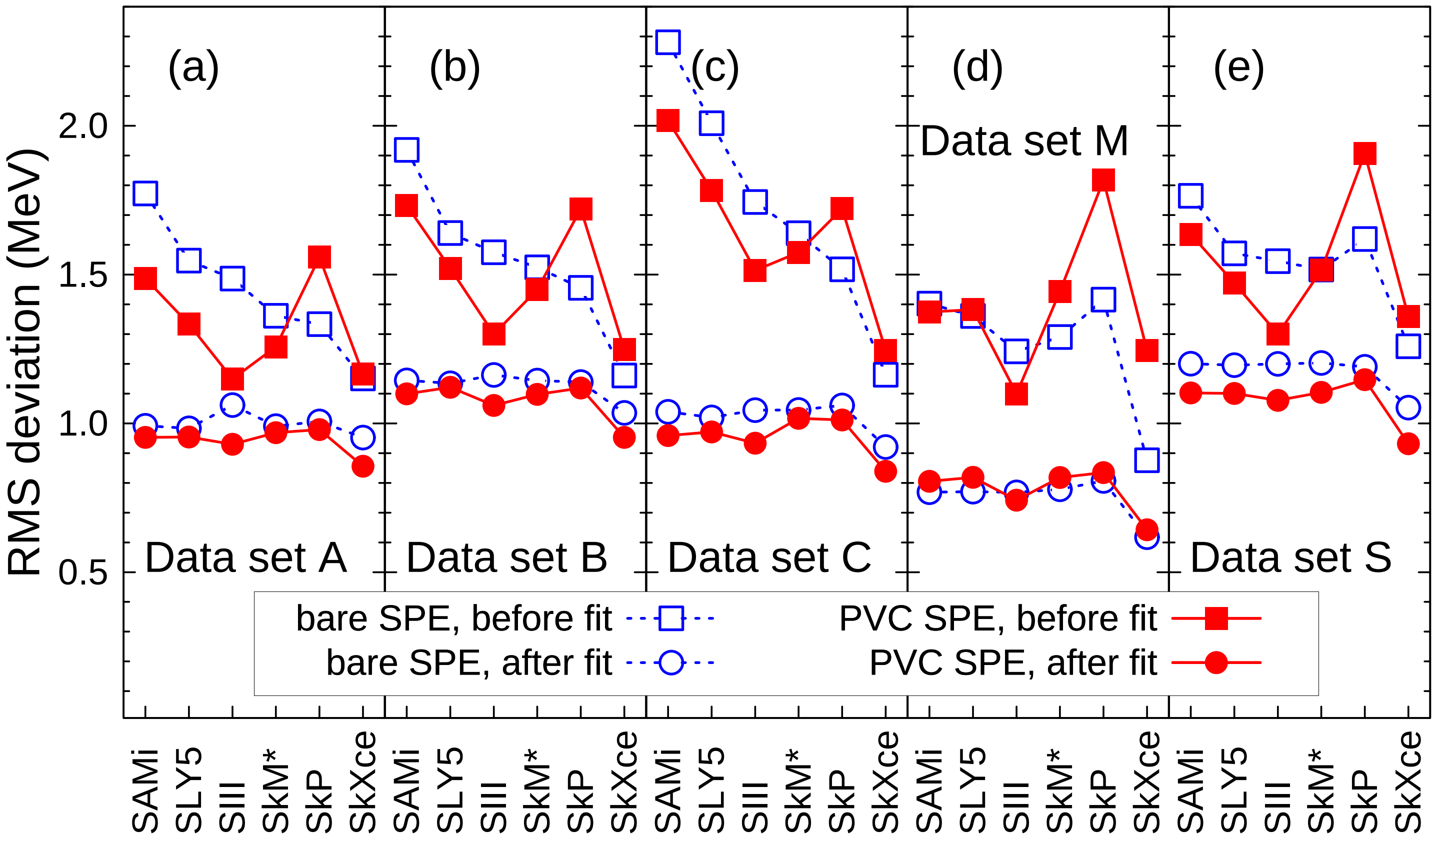


Figure 11: (Color online) Similar to Fig. 5 of the paper, but with Skyrme EDF SKXce included.

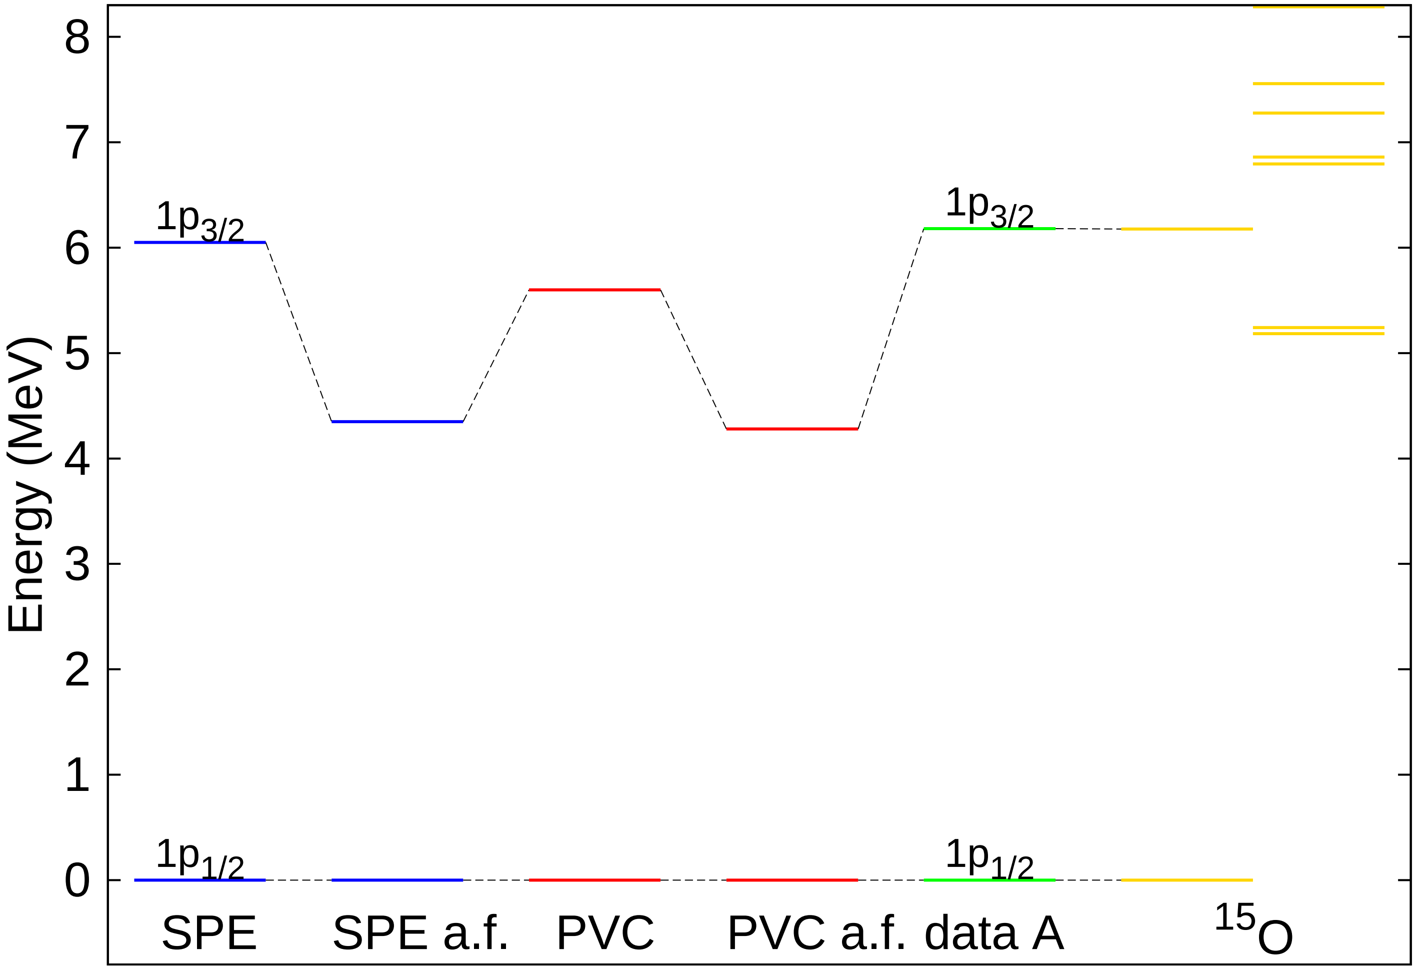


Figure 12: (Color online). Single-particle energies in $^{15}$O. From left to right, the columns correspond to: calculated bare SPEs, calculated bare SPEs after fit (a.f.) as described in the paper, PVC-corrected SPEs, PVC-corrected SPEs after fit, empirical SPEs of data set A, and experimental energies. The experimental energies are split into two columns: the left column contains states connected by dashed lines to those states of the empirical data set A that have identical spins and parities, whereas the right column contains all the remaining states.

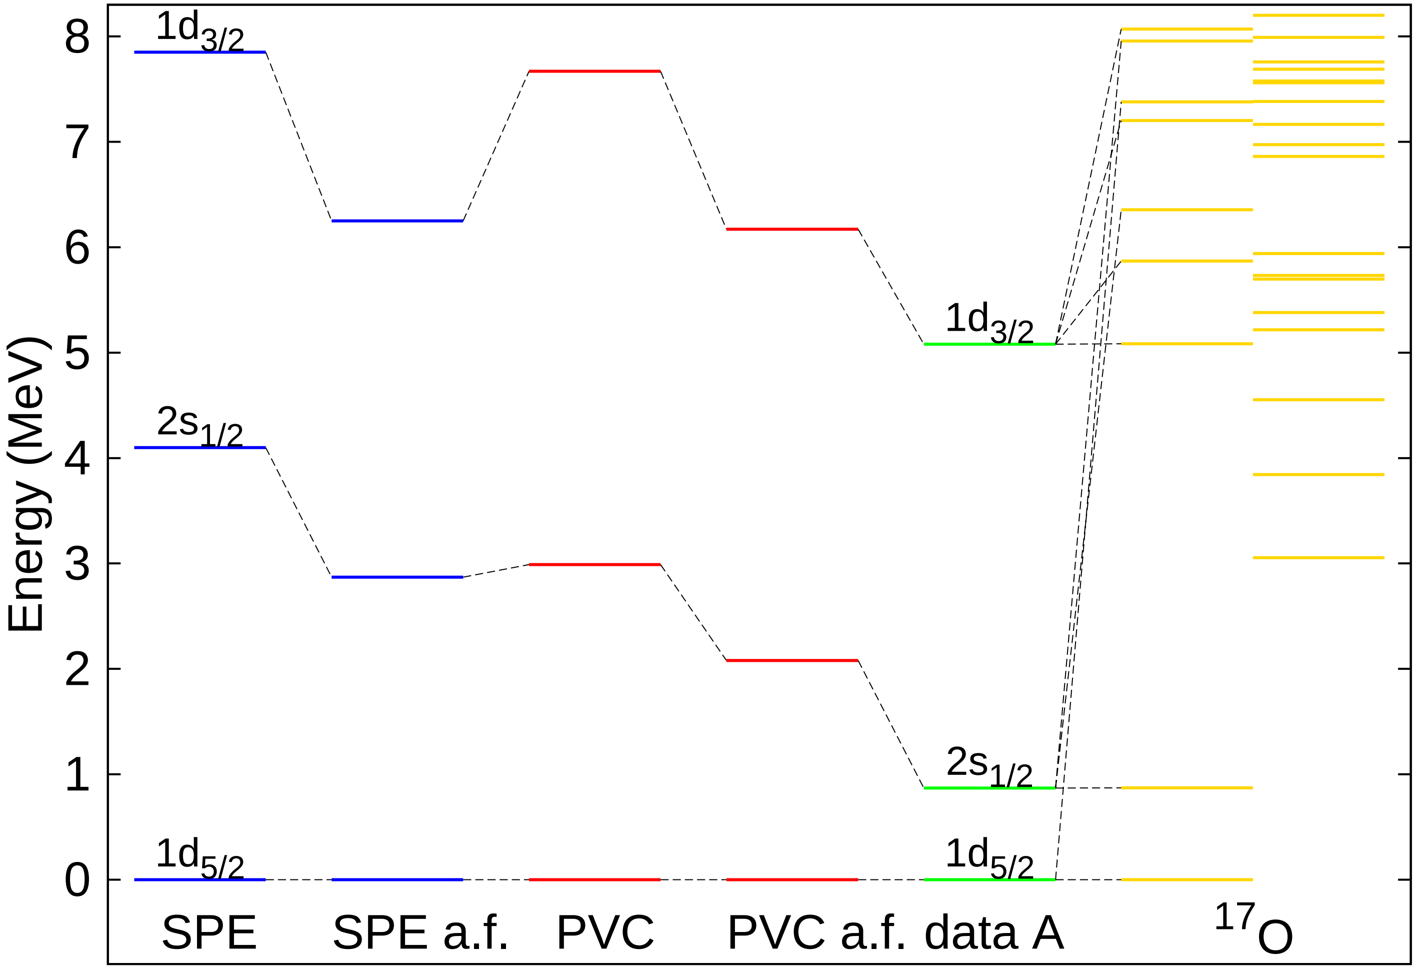


Figure 13: (Color online). Similar to Fig. 12, but for $^{17}$O.

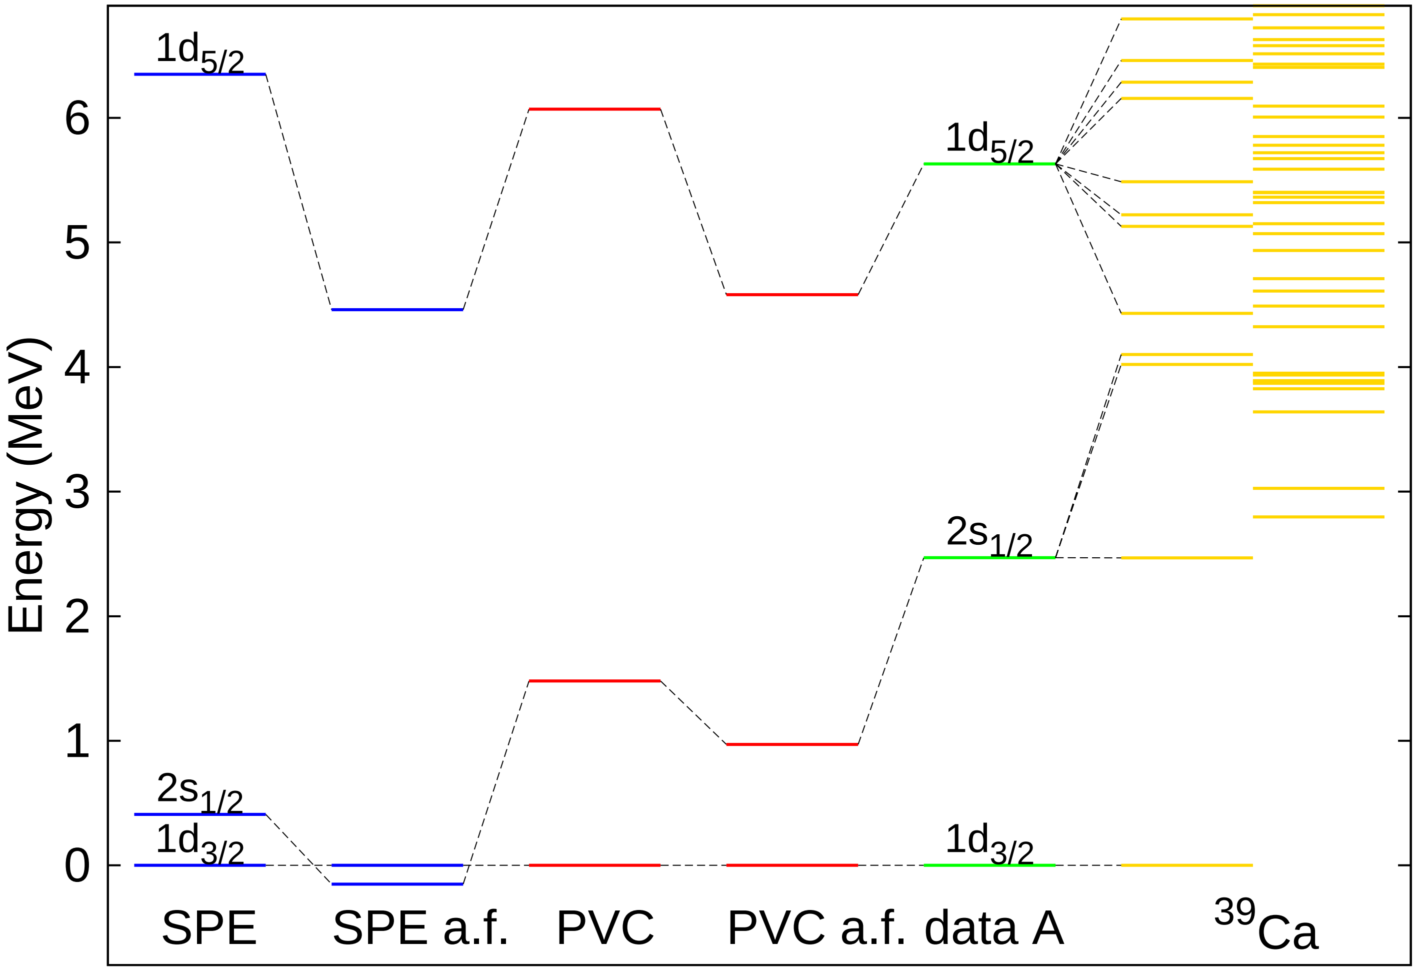


Figure 14: (Color online). Similar to Fig. 12, but for $^{39}$Ca.

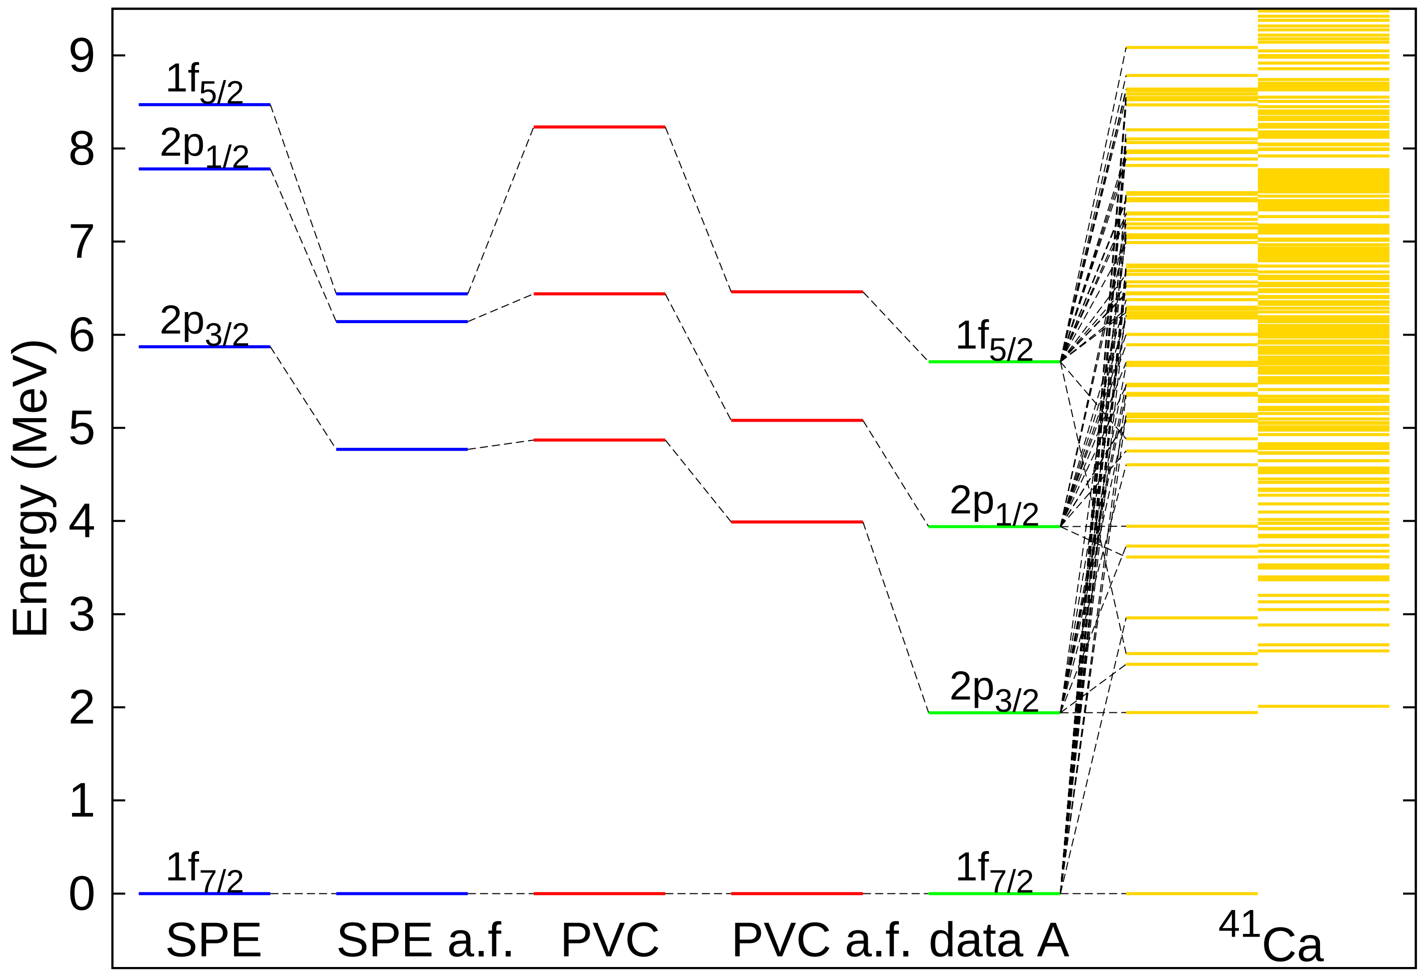


Figure 15: (Color online). Similar to Fig. 12, but for $^{41}$Ca.

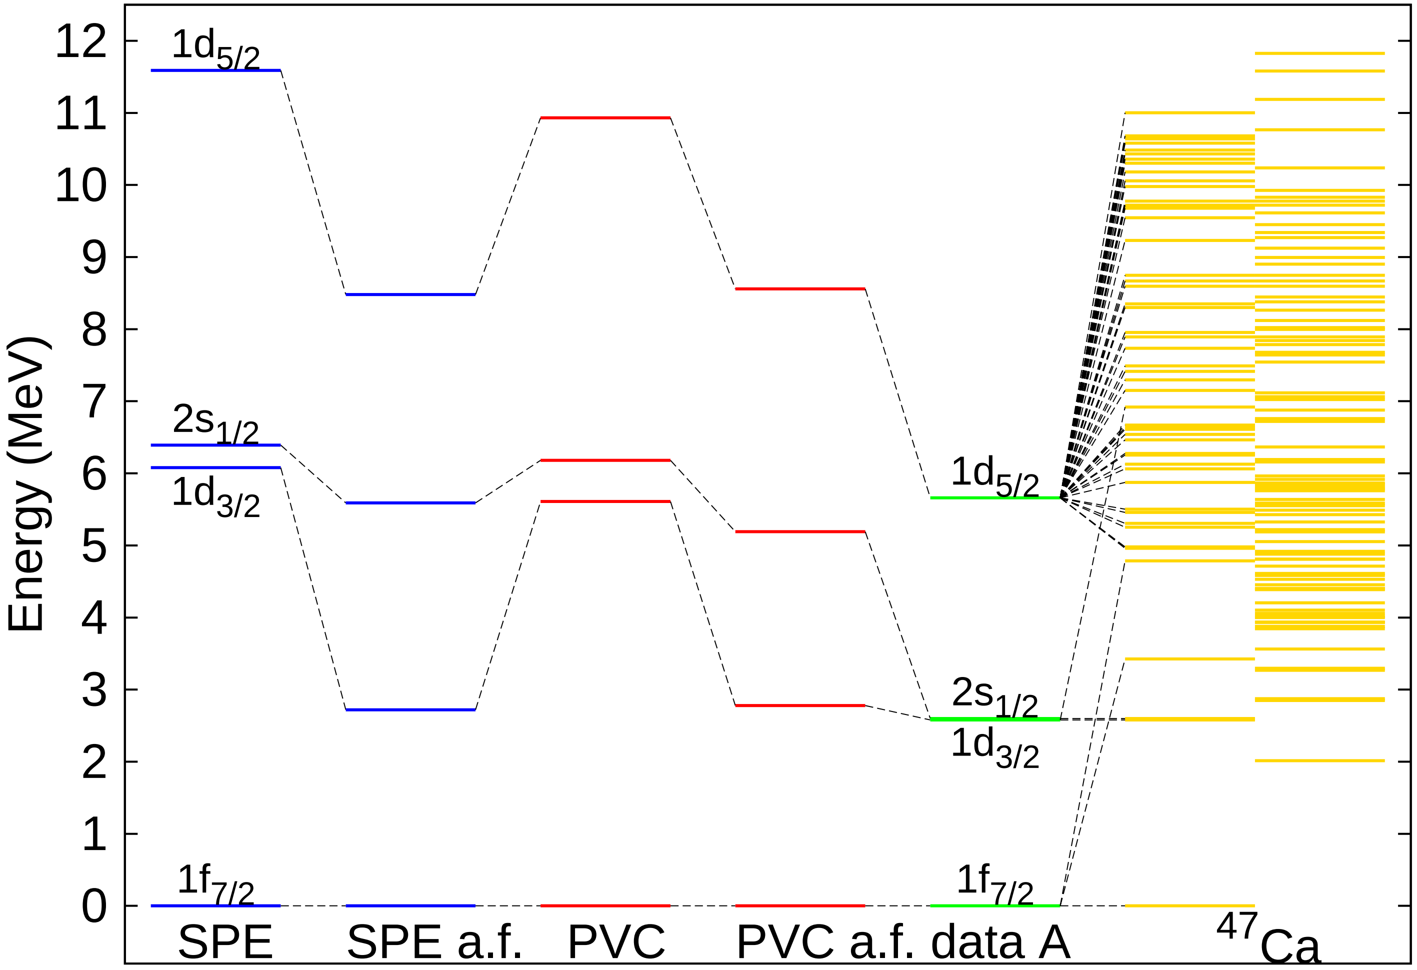


Figure 16: (Color online). Similar to Fig. 12, but for $^{47}$Ca.

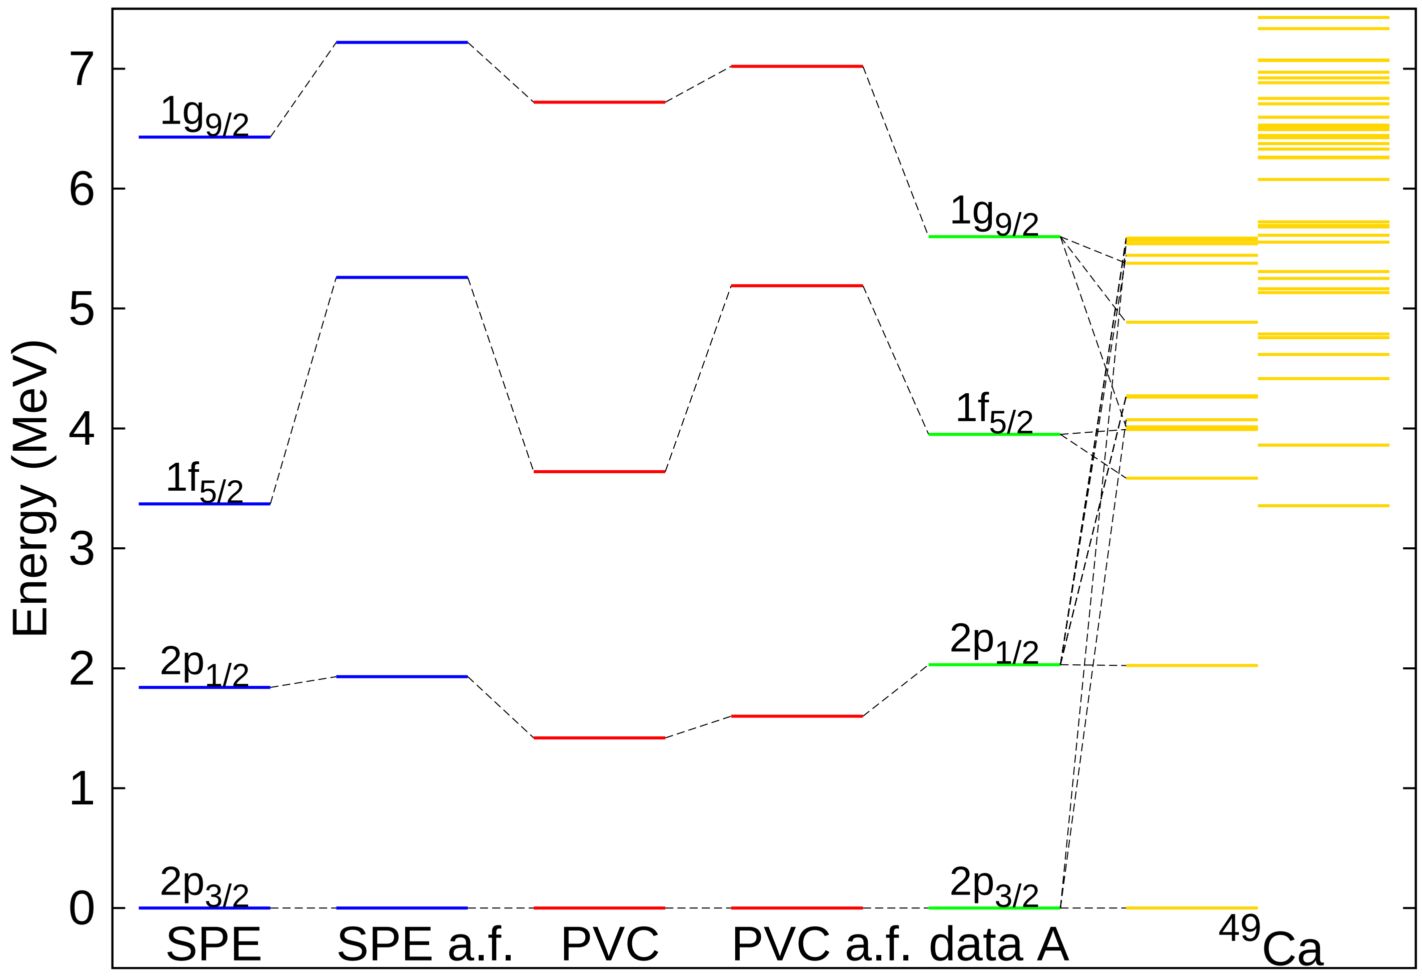


Figure 17: (Color online). Similar to Fig. 12, but for $^{49}$Ca.

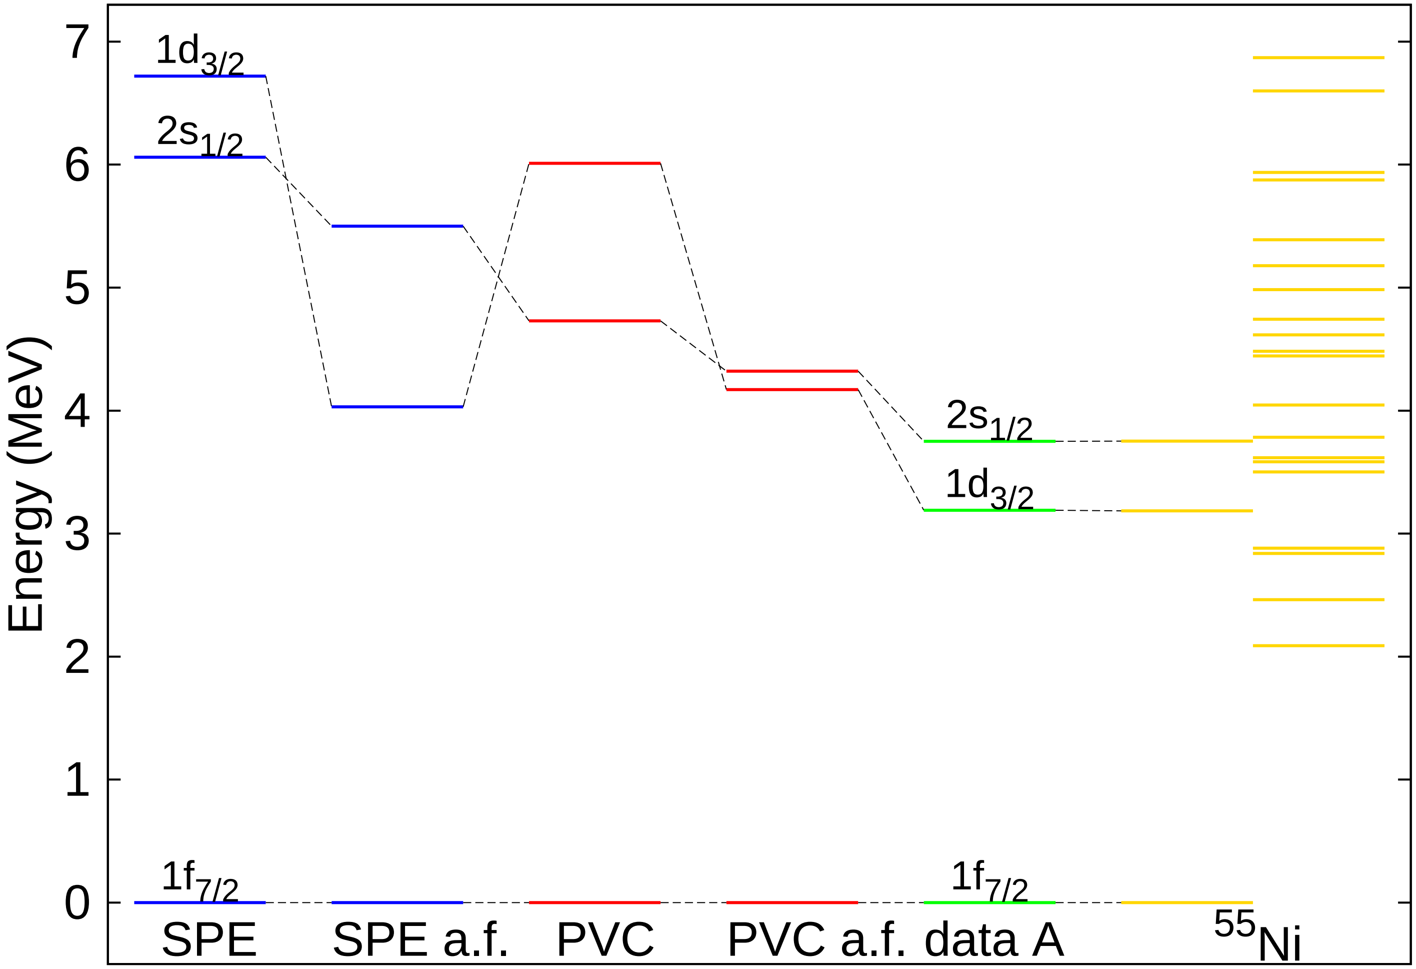


Figure 18: (Color online). Similar to Fig. 12, but for $^{55}$Ni.

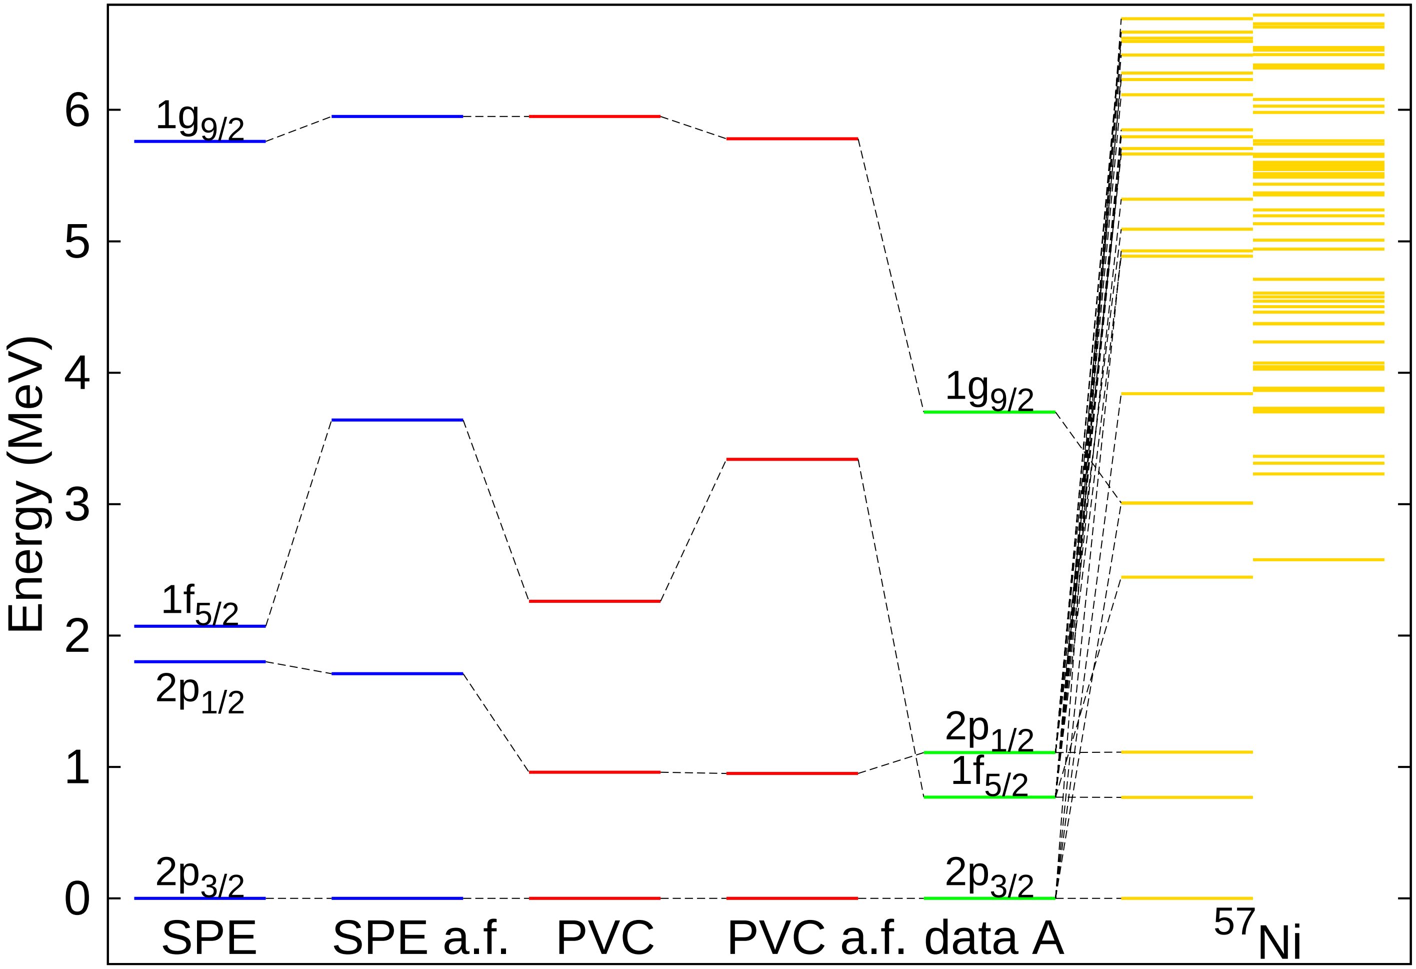


Figure 19: (Color online). Similar to Fig. 12, but for $^{57}$Ni.

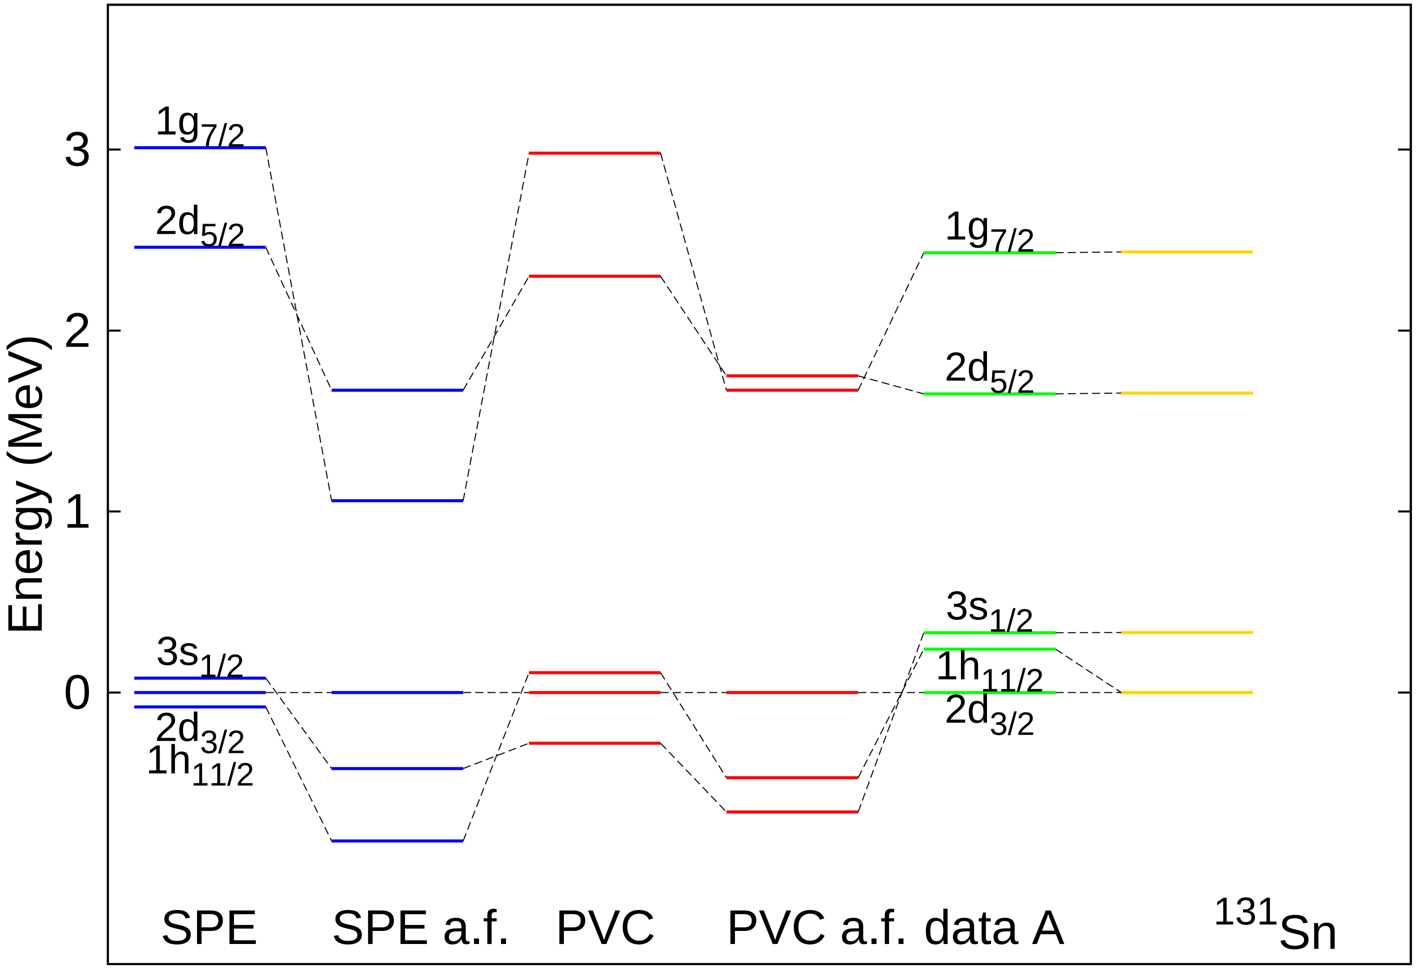


Figure 20: (Color online). Similar to Fig. 12, but for $^{131}$Sn.

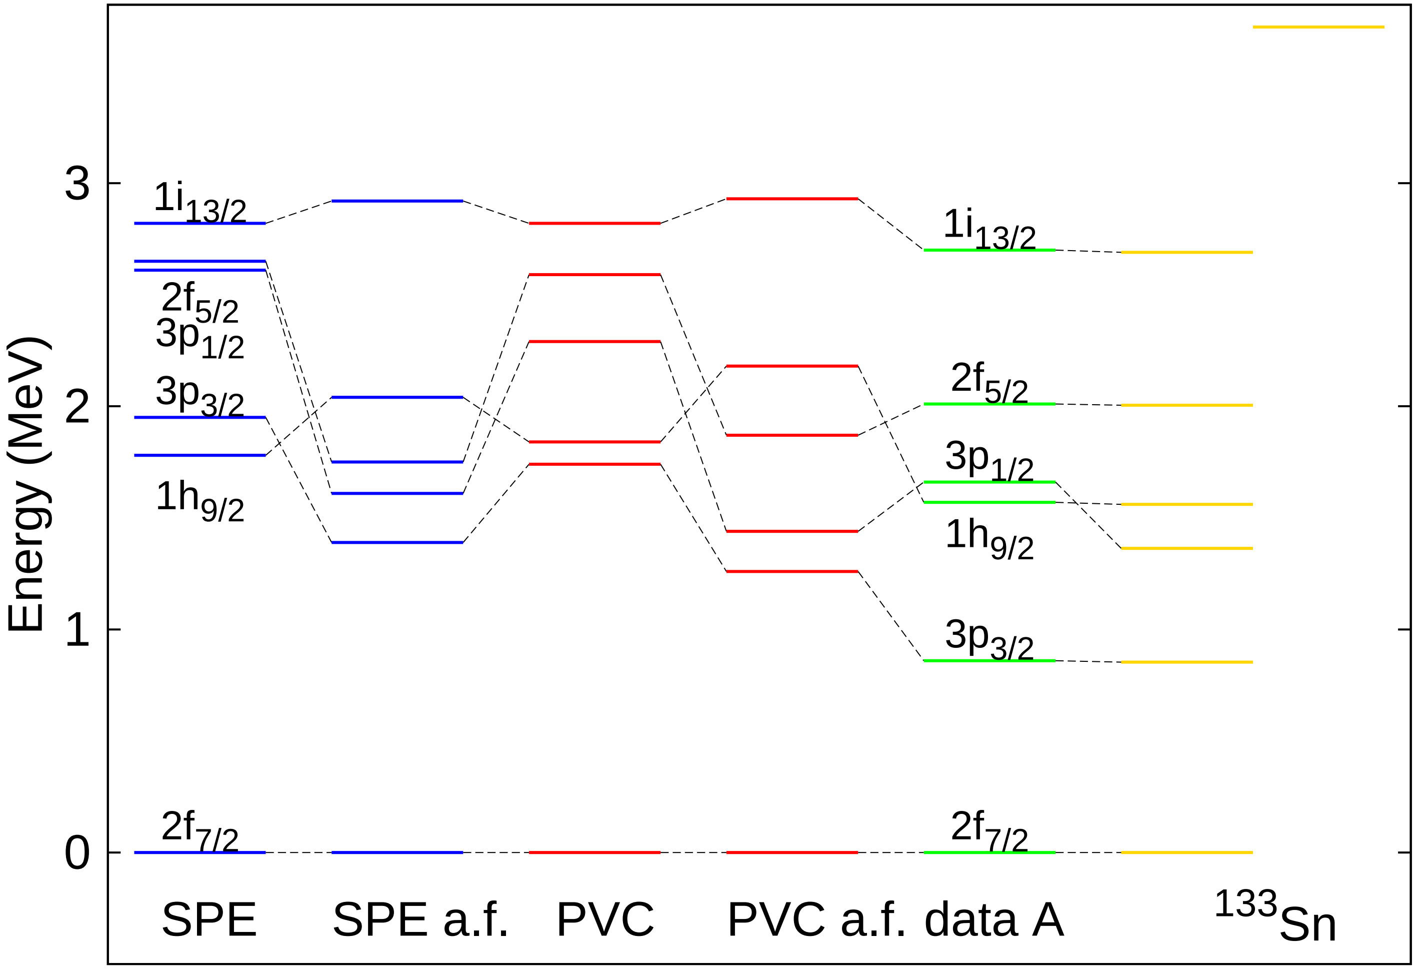


Figure 21: (Color online). Similar to Fig. 12, but for $^{133}$Sn.

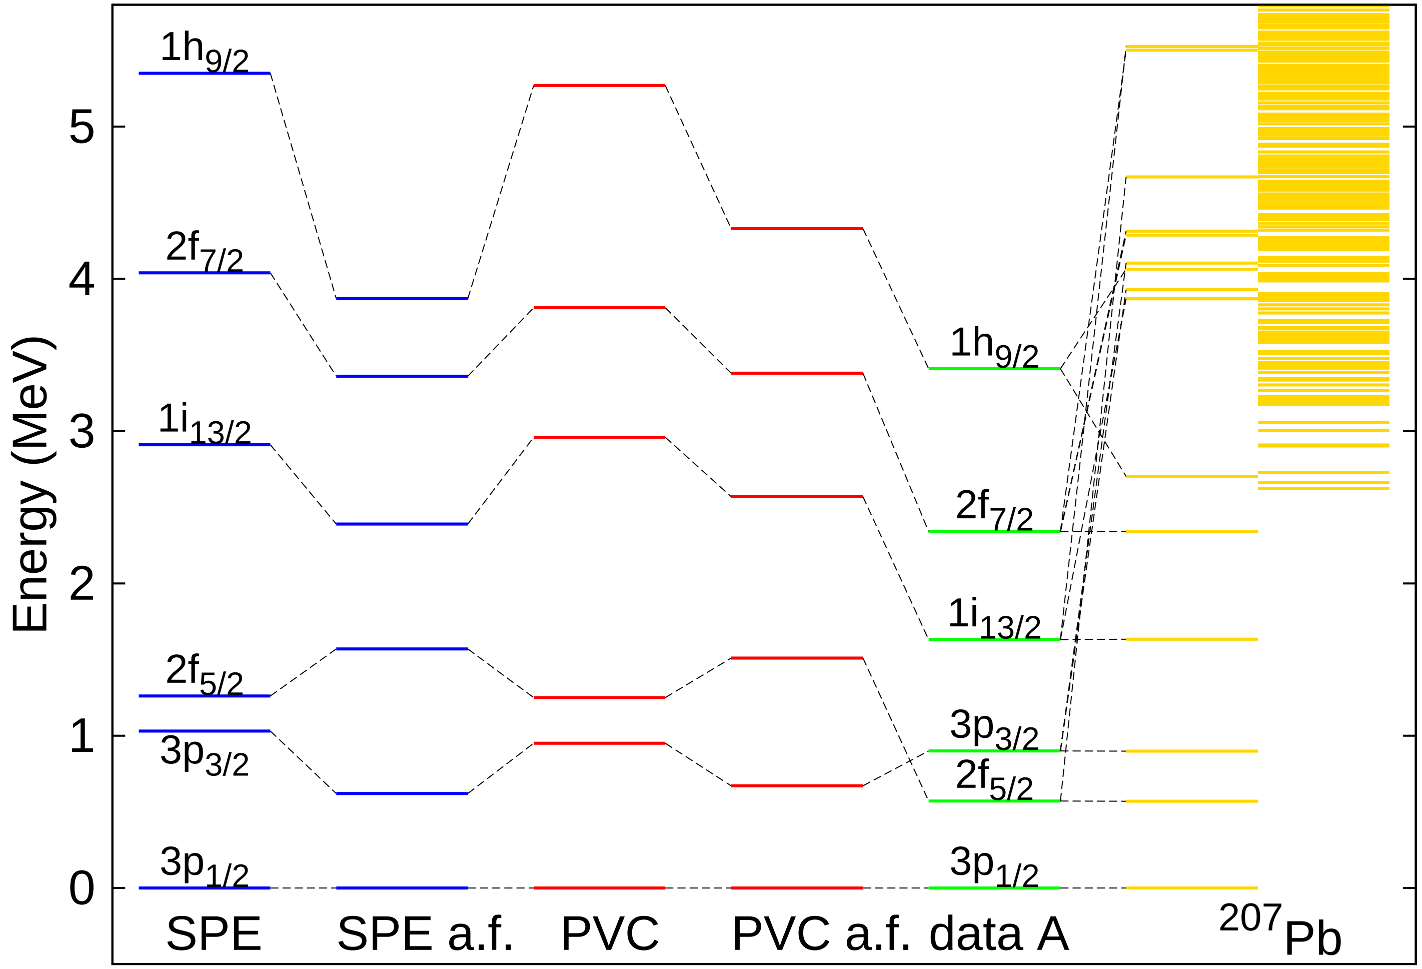


Figure 22: (Color online). Similar to Fig. 12, but for $^{207}$Pb.

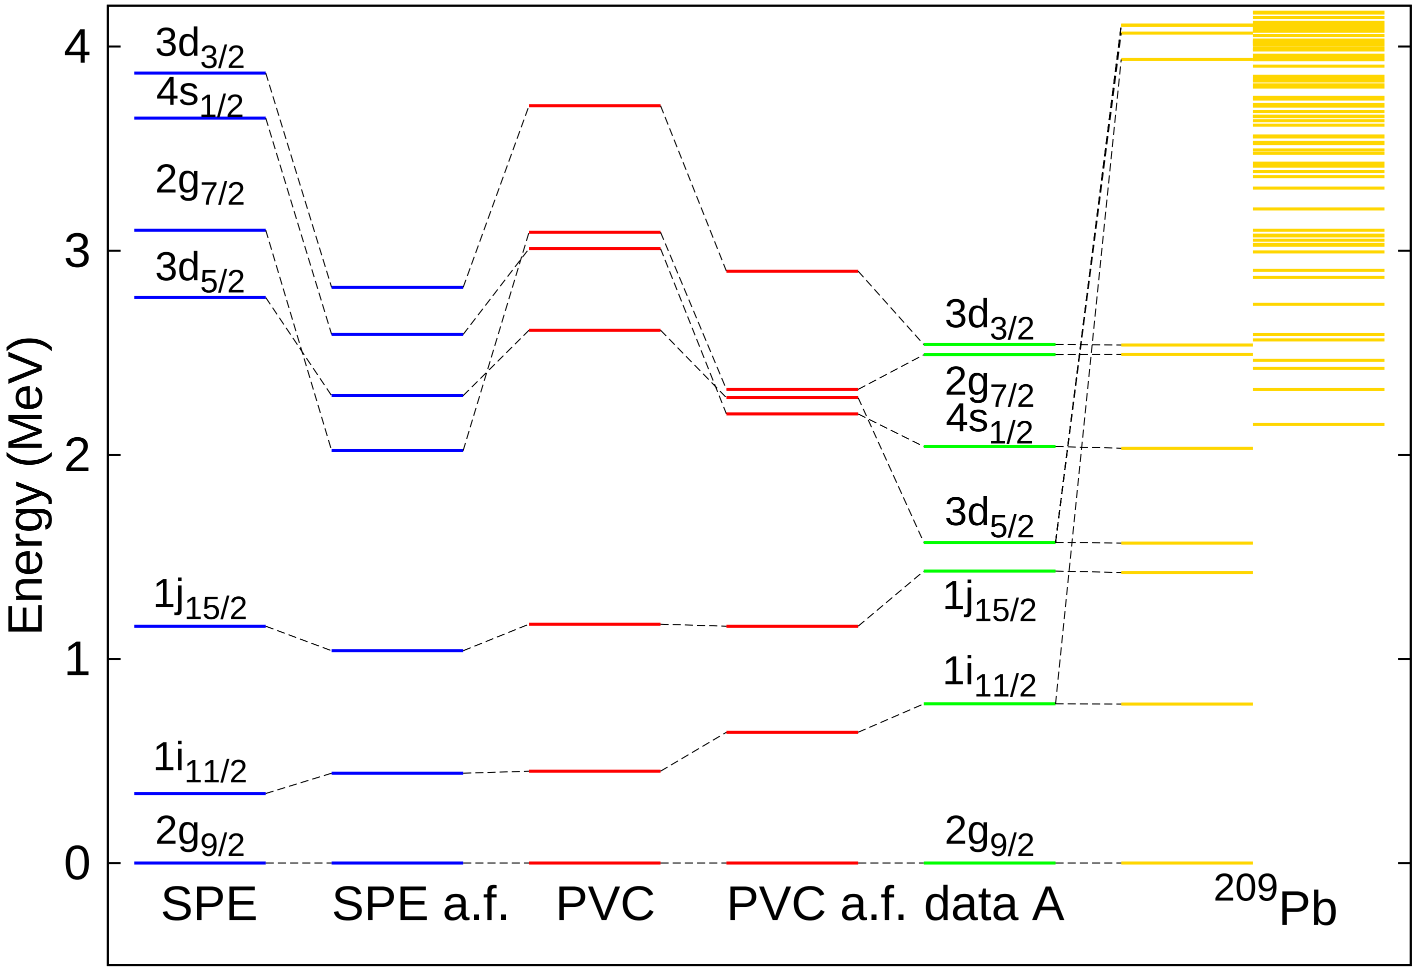


Figure 23: (Color online). Similar to Fig. 12, but for $^{209}$Pb.

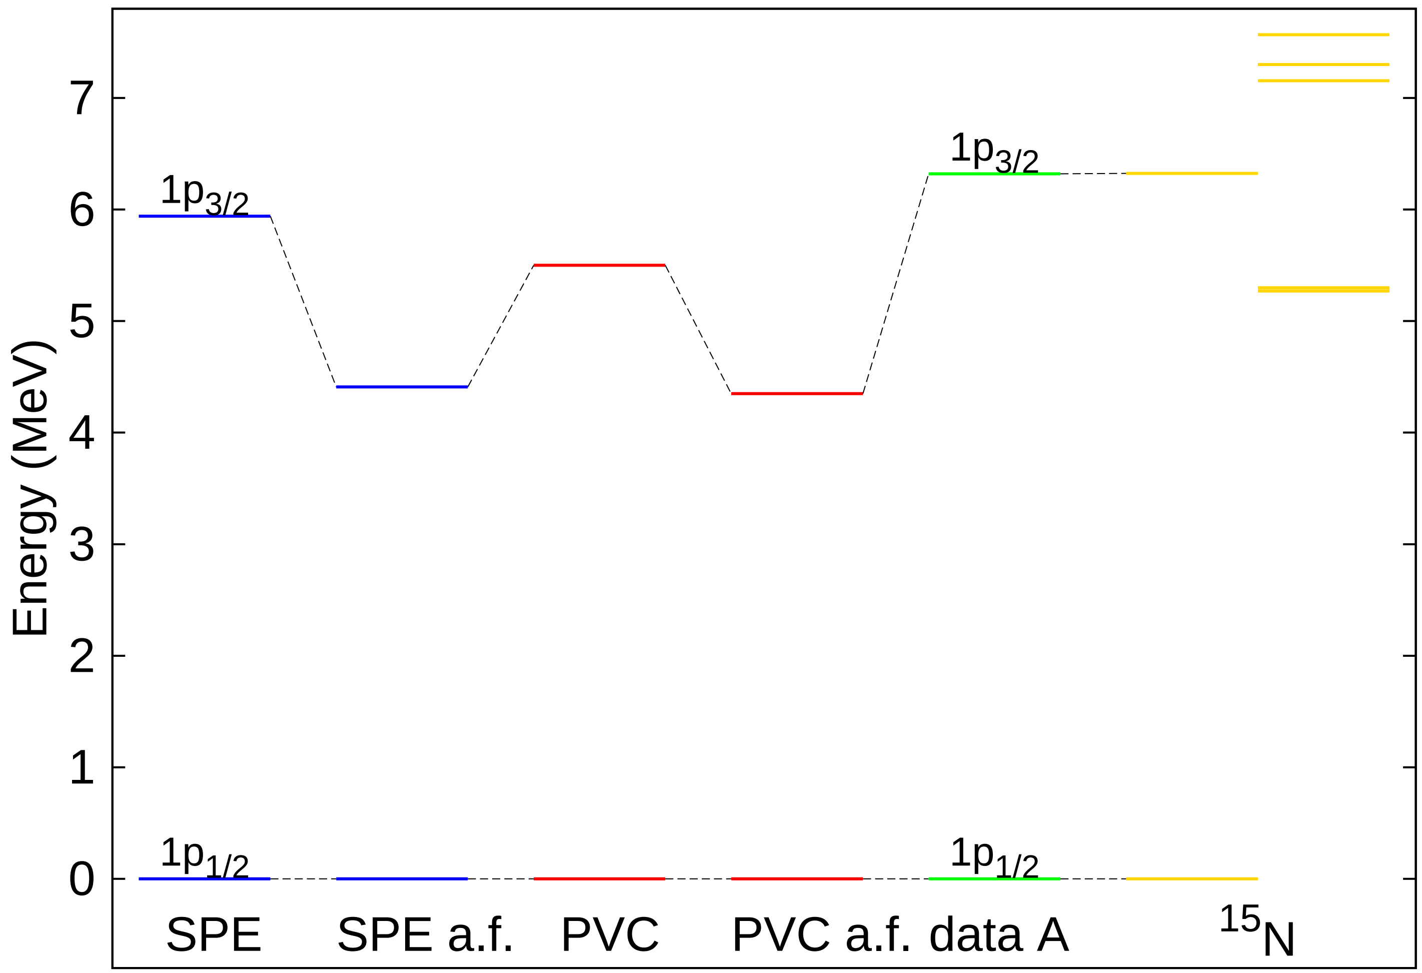


Figure 24: (Color online). Similar to Fig. 12, but for $^{15}$N.

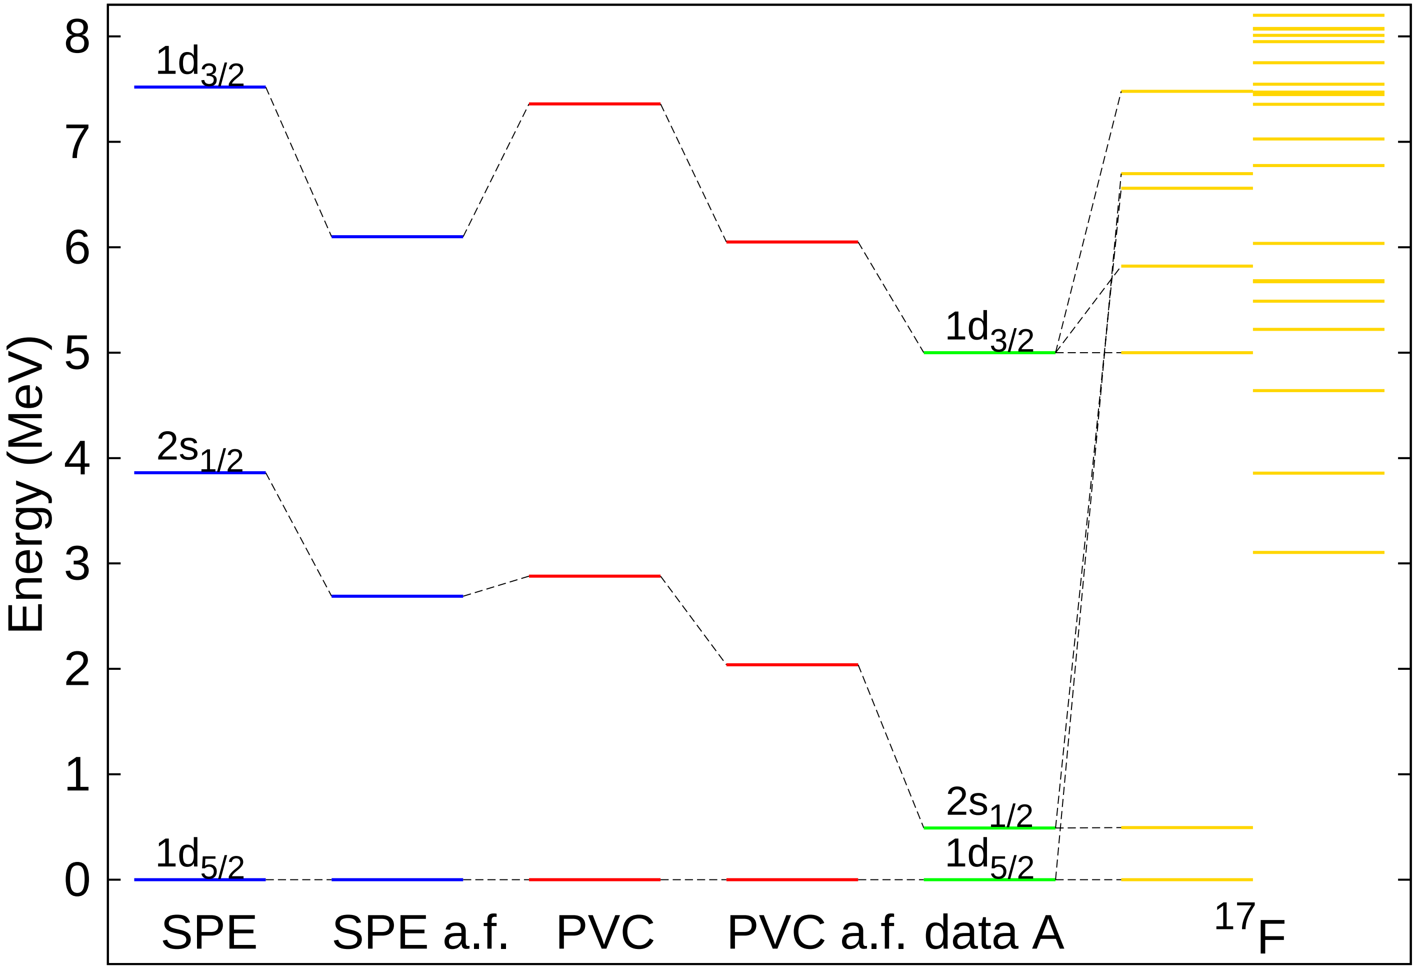


Figure 25: (Color online). Similar to Fig. 12, but for $^{17}$F.

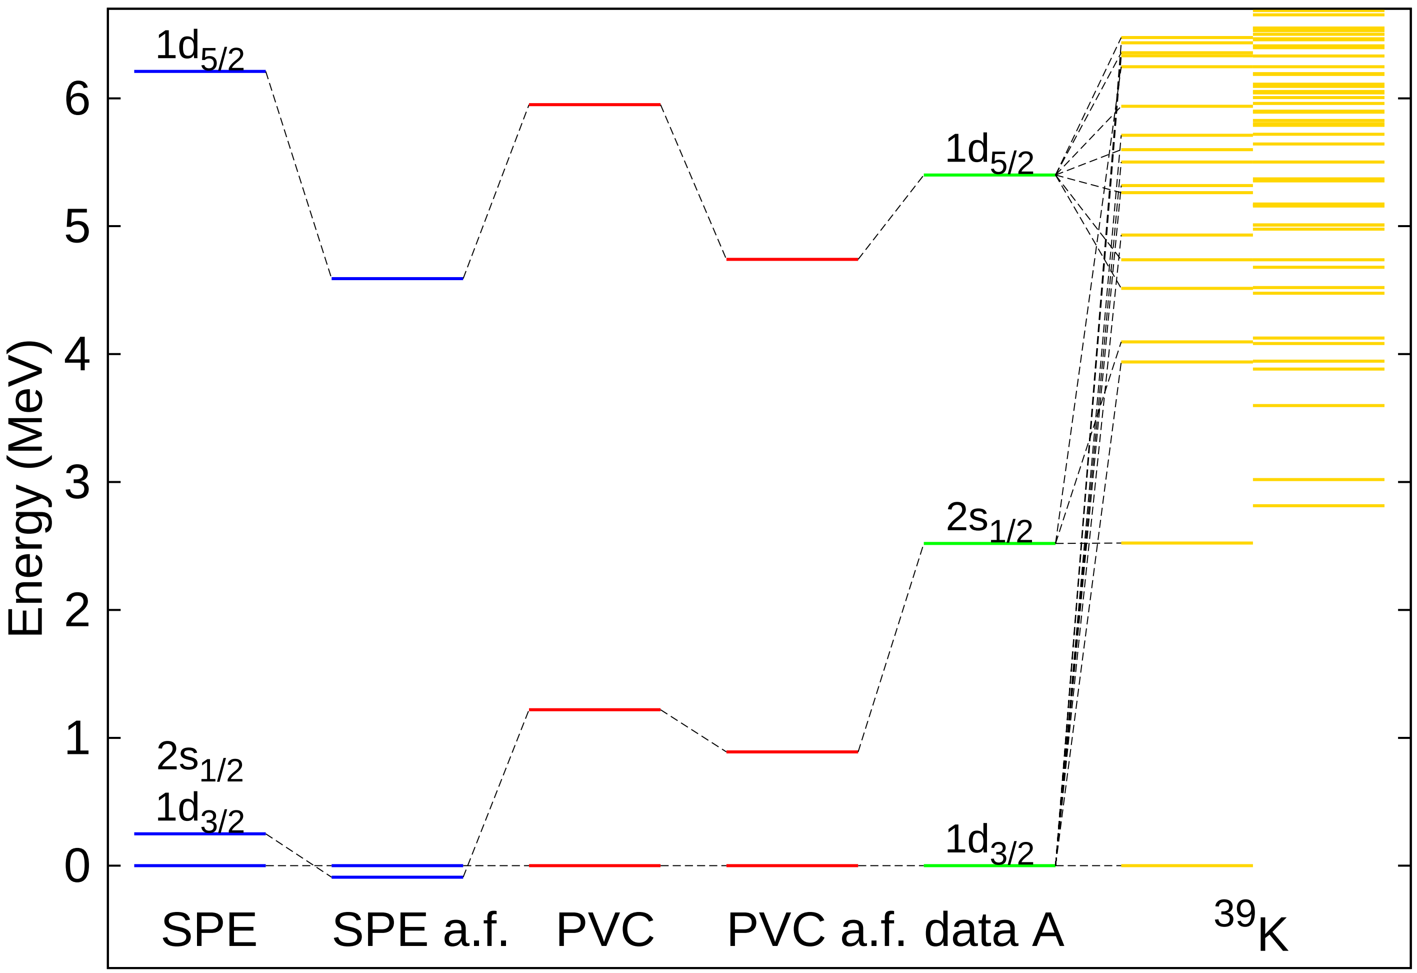


Figure 26: (Color online). Similar to Fig. 12, but for $^{39}$K.

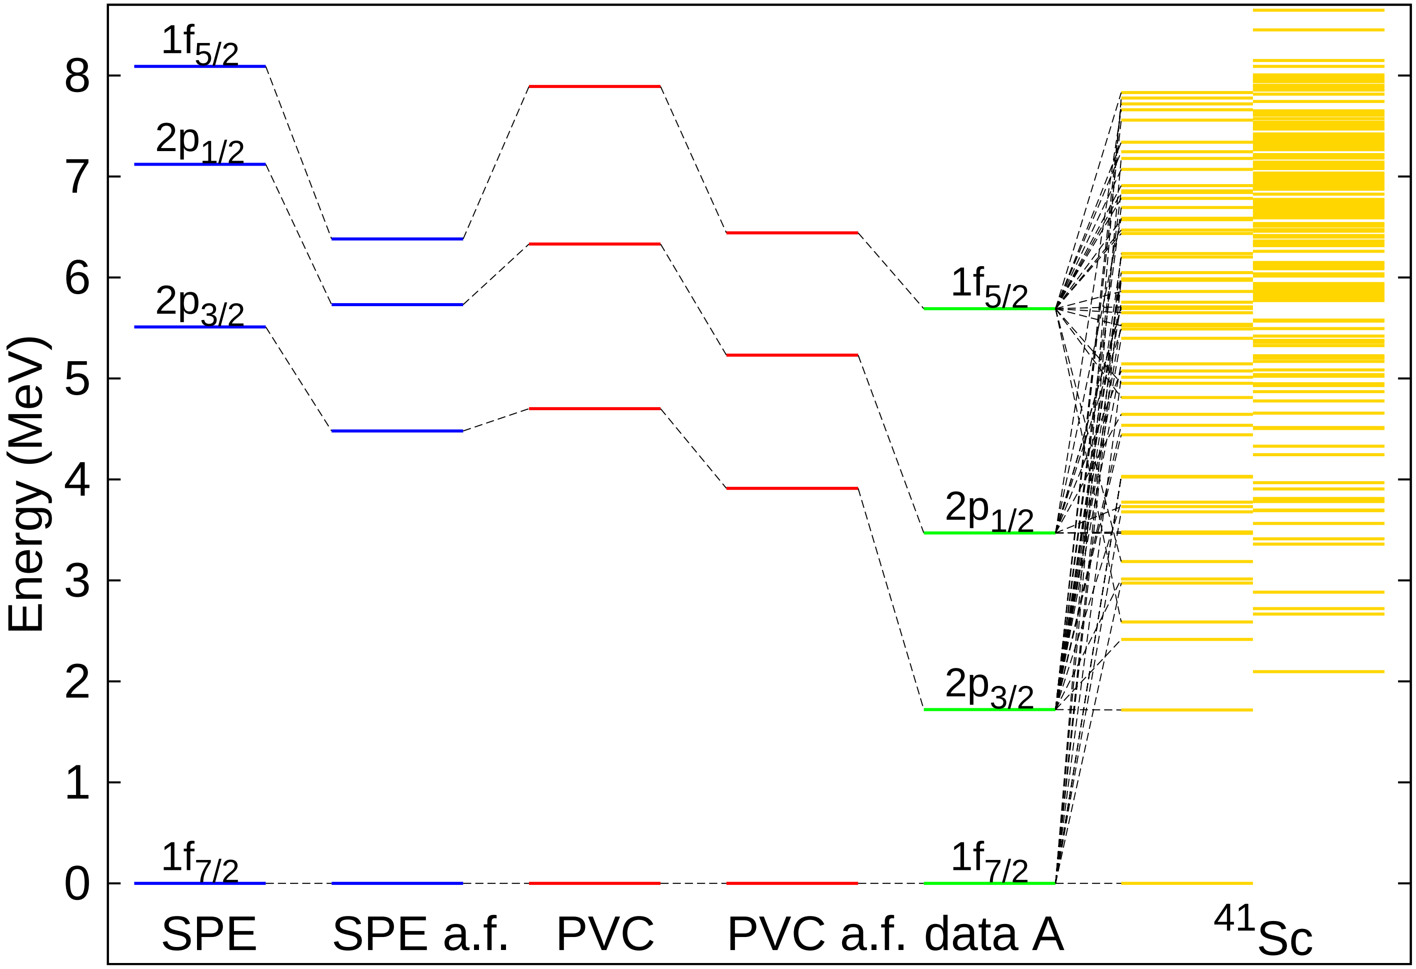


Figure 27: (Color online). Similar to Fig. 12, but for $^{41}$Sc.

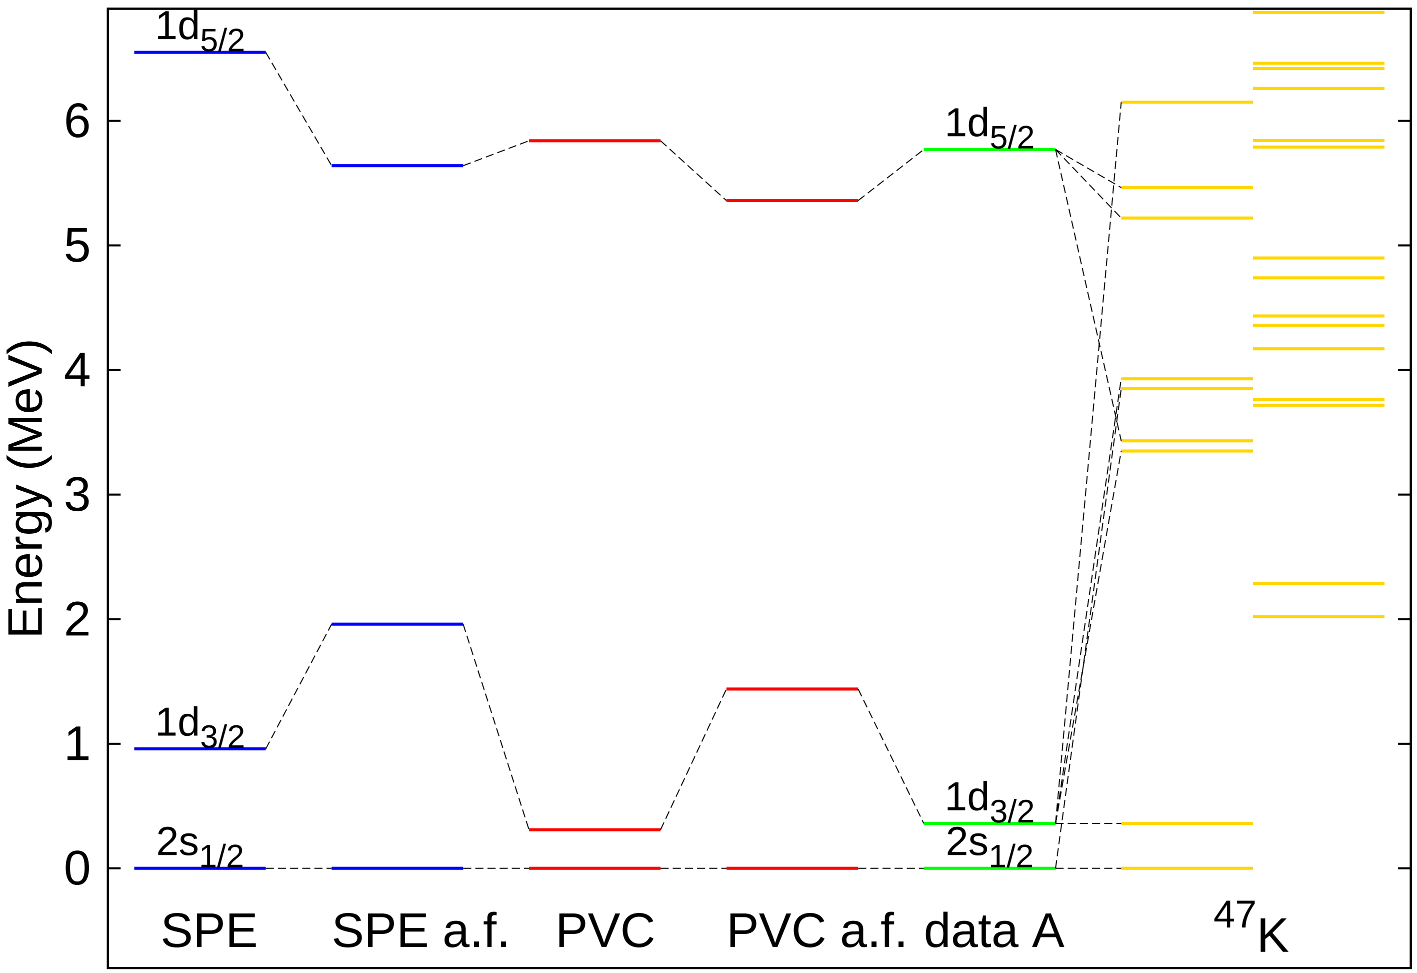


Figure 28: (Color online). Similar to Fig. 12, but for $^{47}$K.

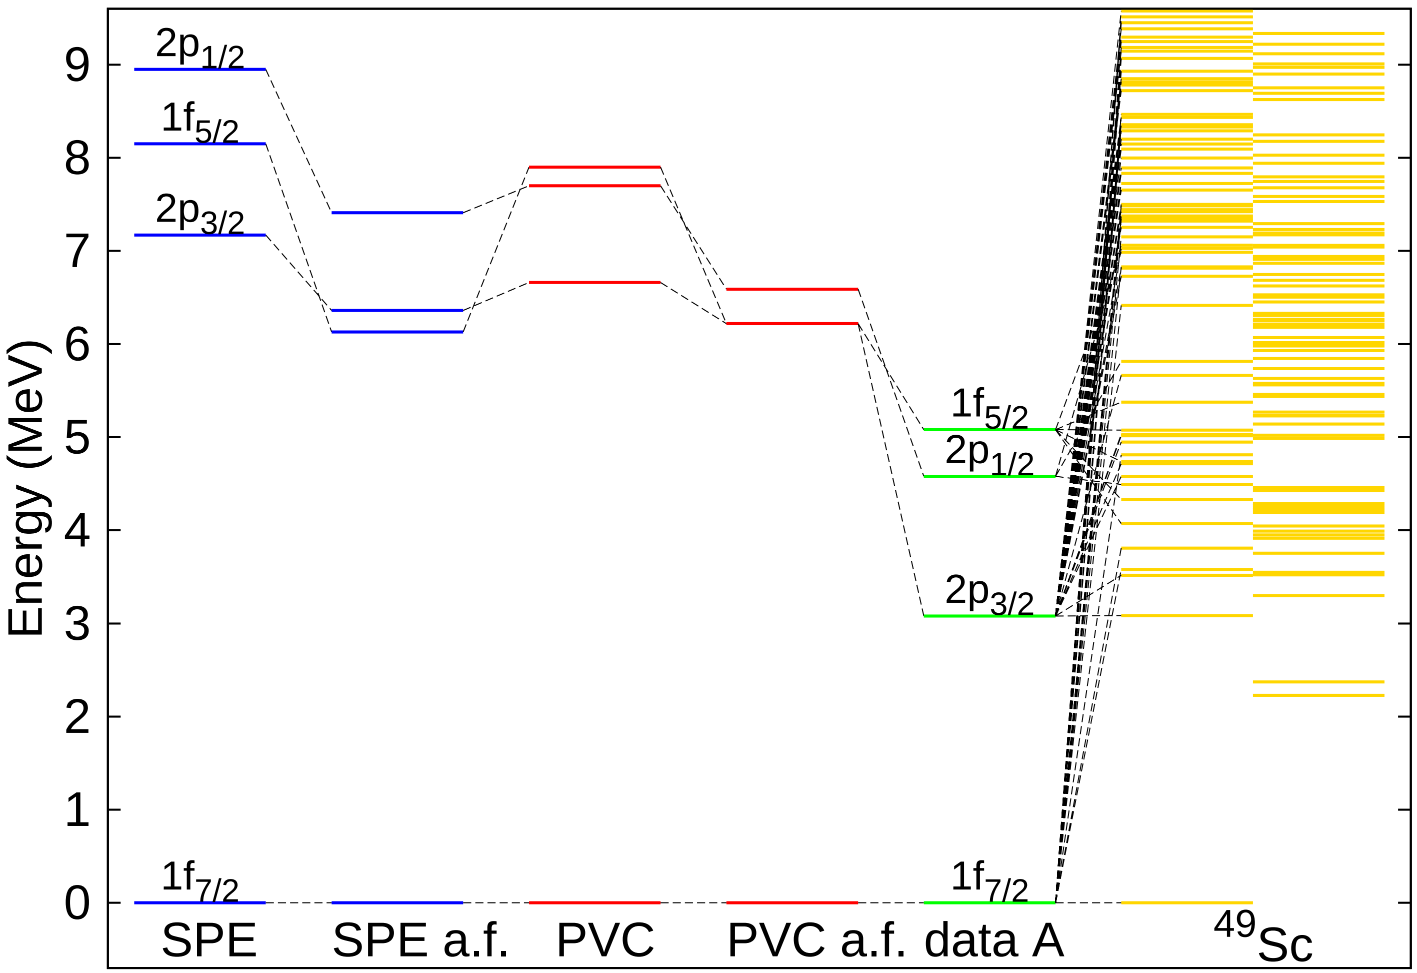


Figure 29: (Color online). Similar to Fig. 12, but for $^{49}$Sc.

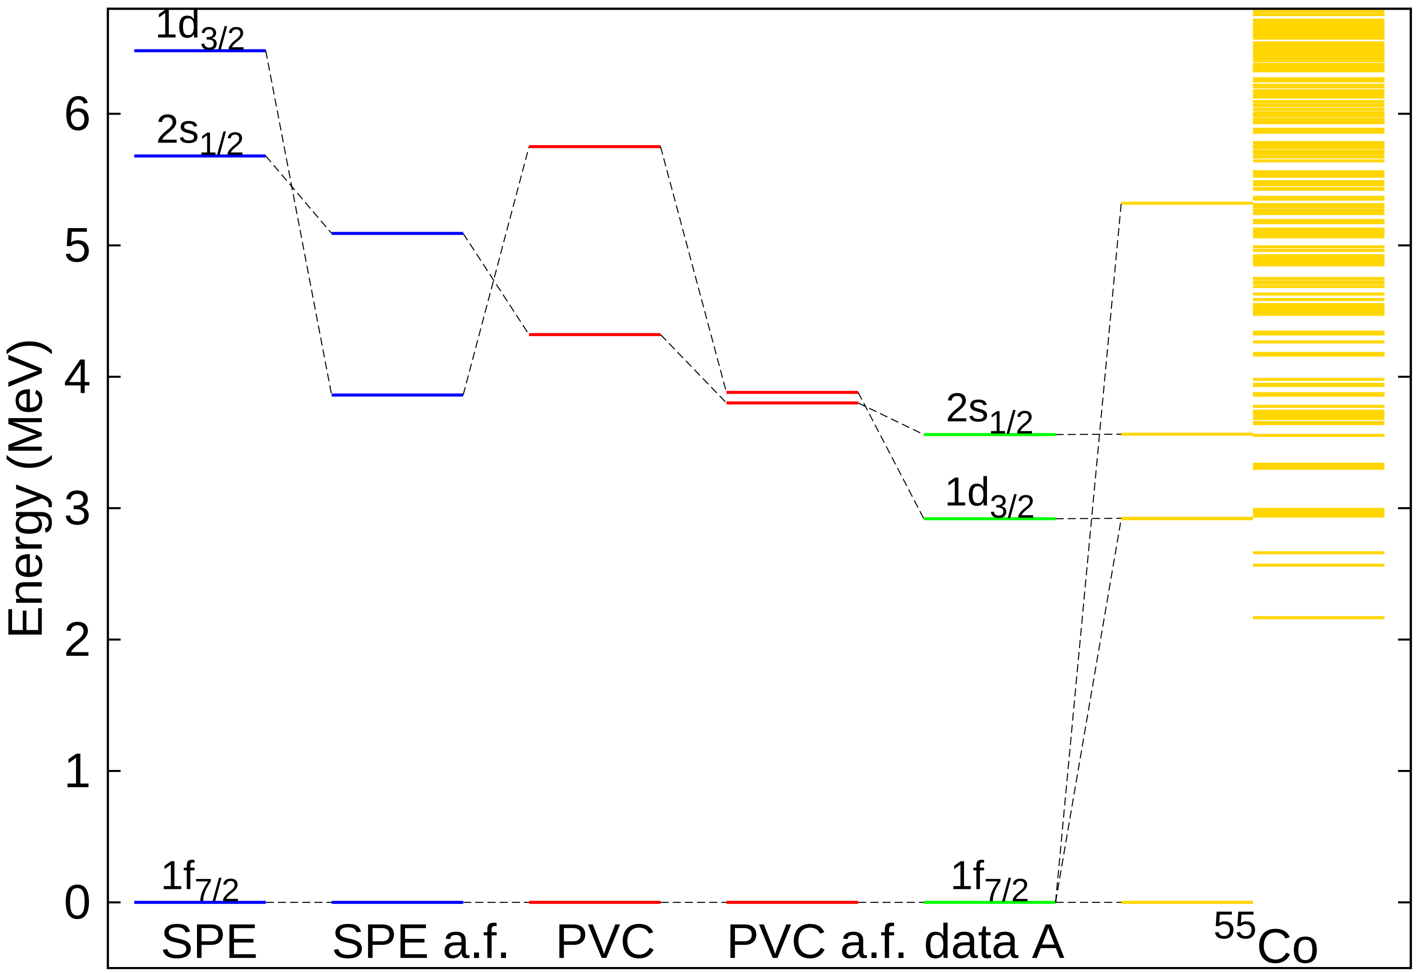


Figure 30: (Color online). Similar to Fig. 12, but for $^{55}$Co.

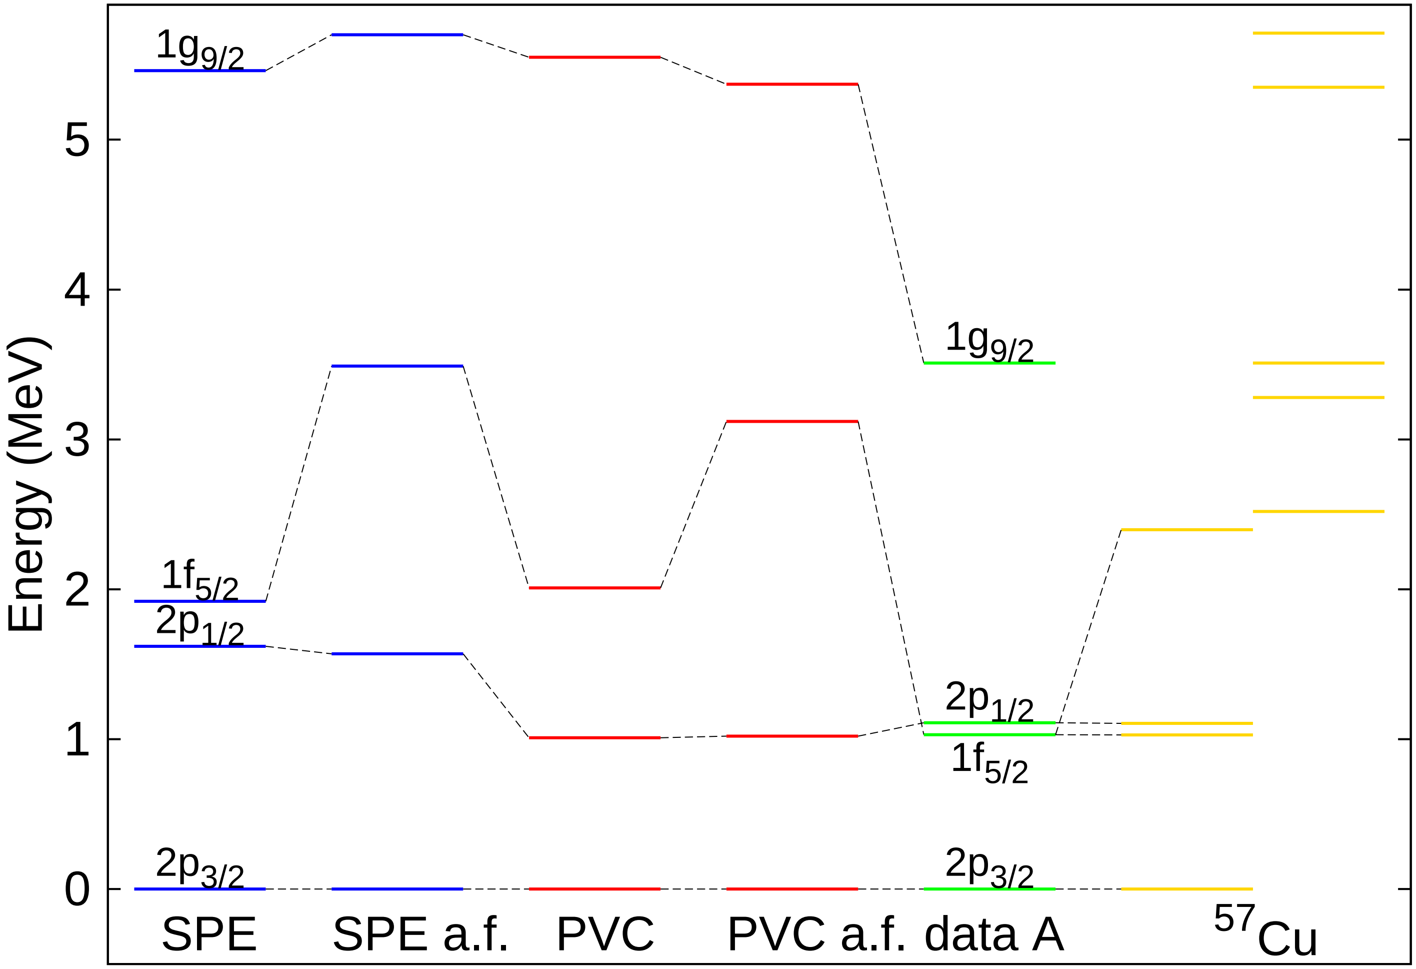


Figure 31: (Color online). Similar to Fig. 12, but for $^{57}$Cu.

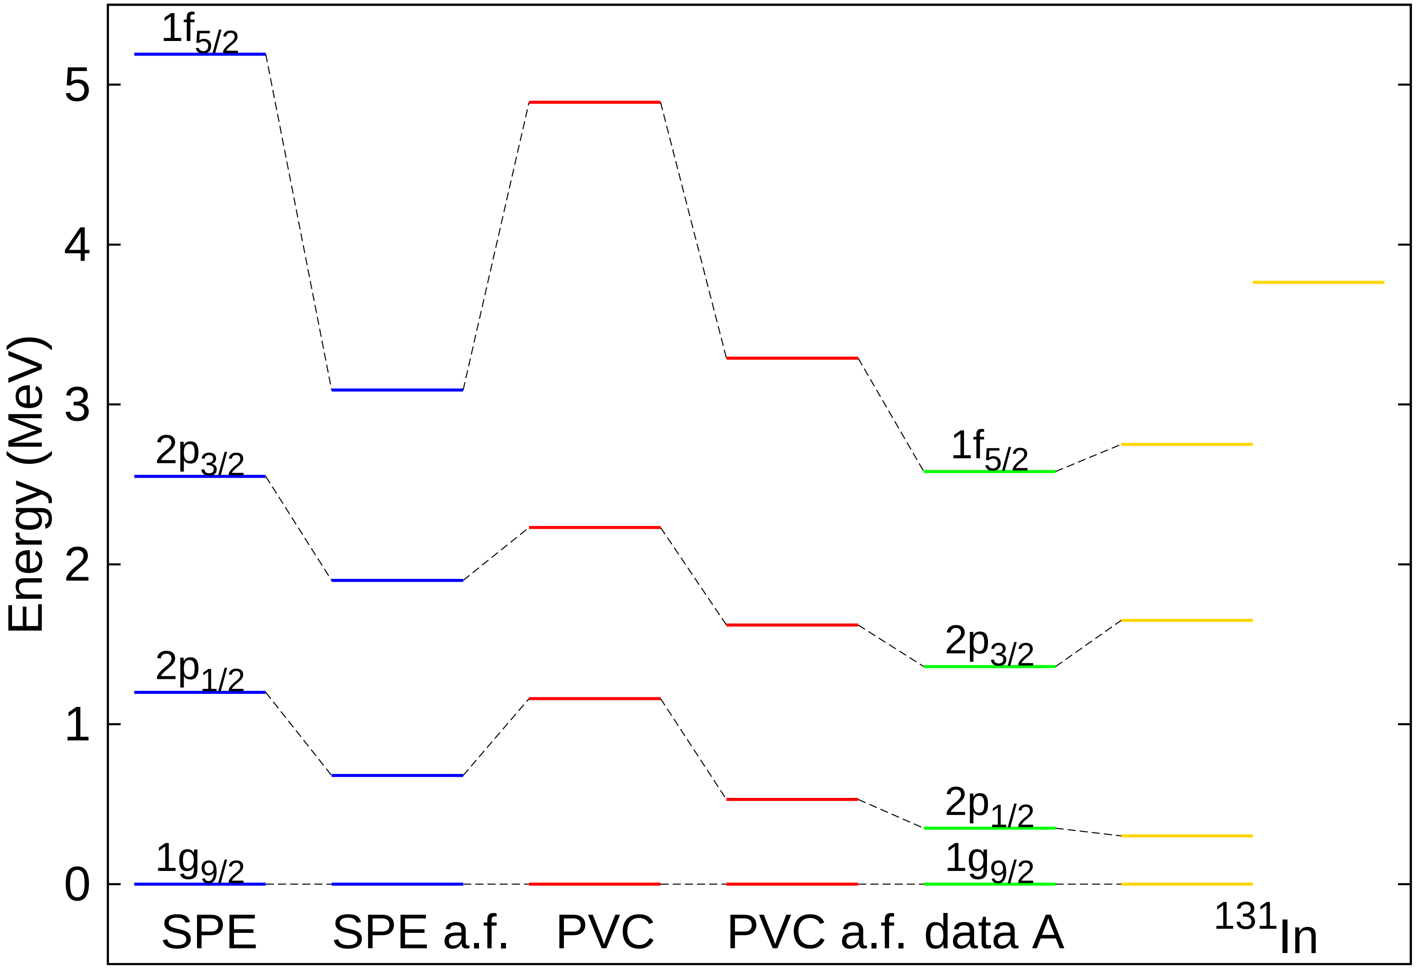


Figure 32: (Color online). Similar to Fig. 12, but for $^{131}$In.

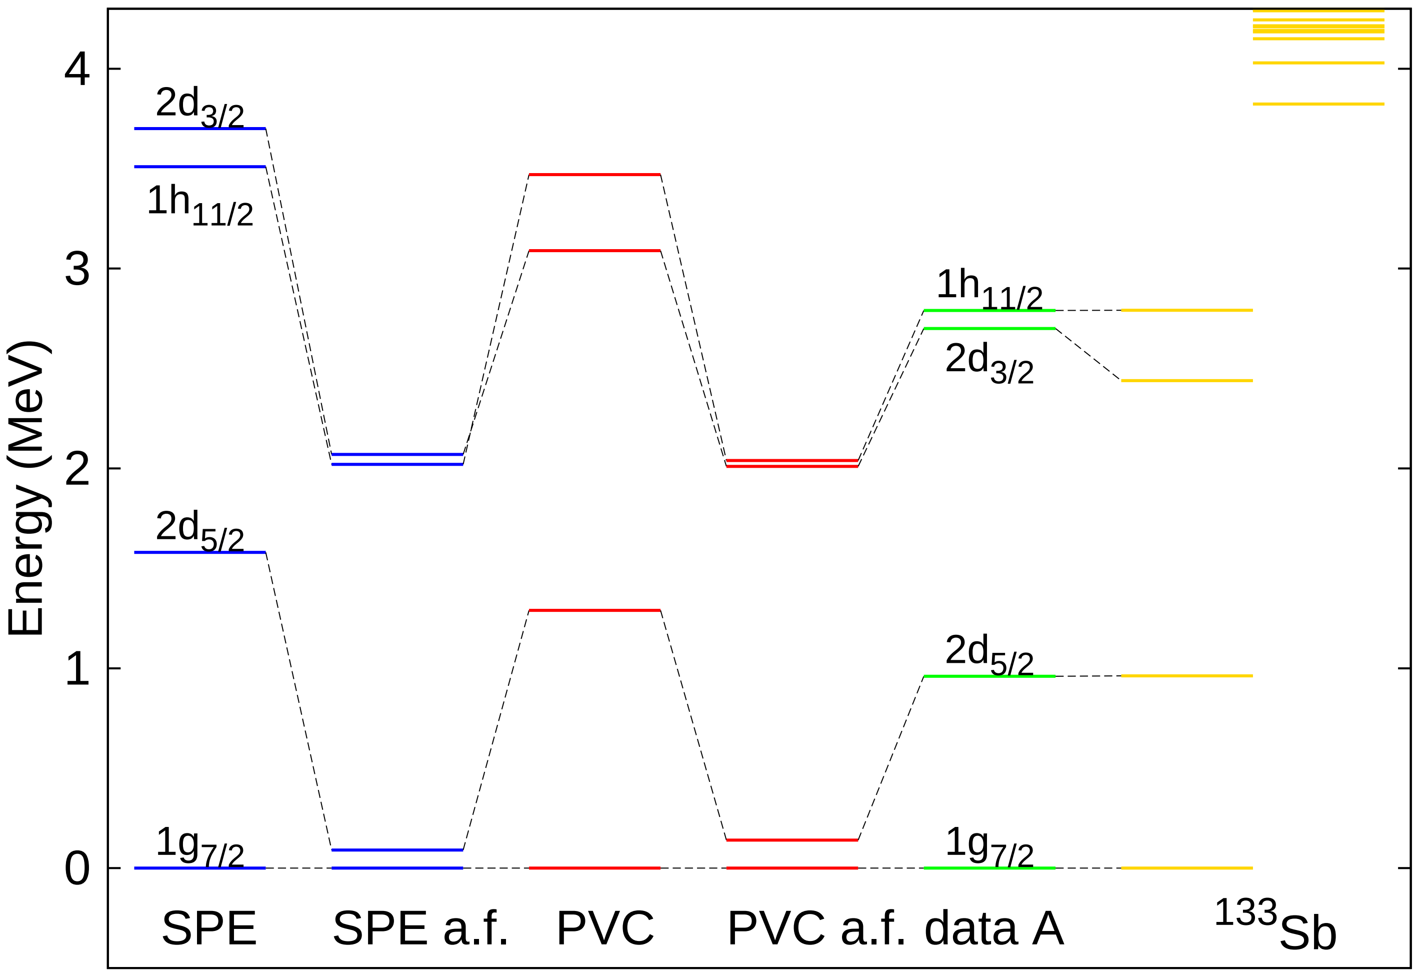


Figure 33: (Color online). Similar to Fig. 12, but for $^{133}$Sb.

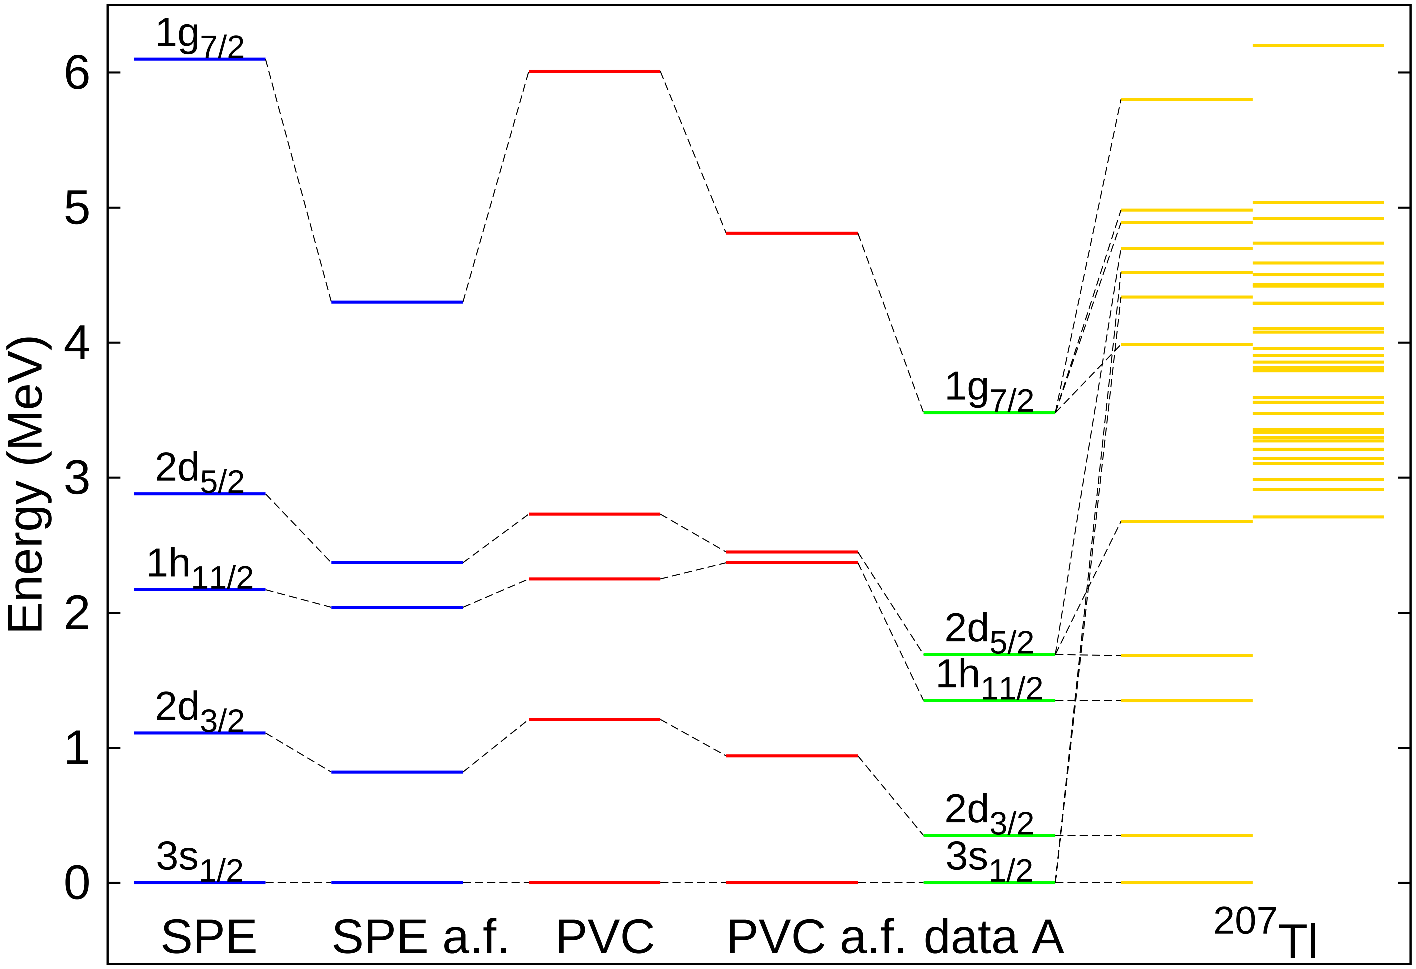


Figure 34: (Color online). Similar to Fig. 12, but for $^{207}$Tl.

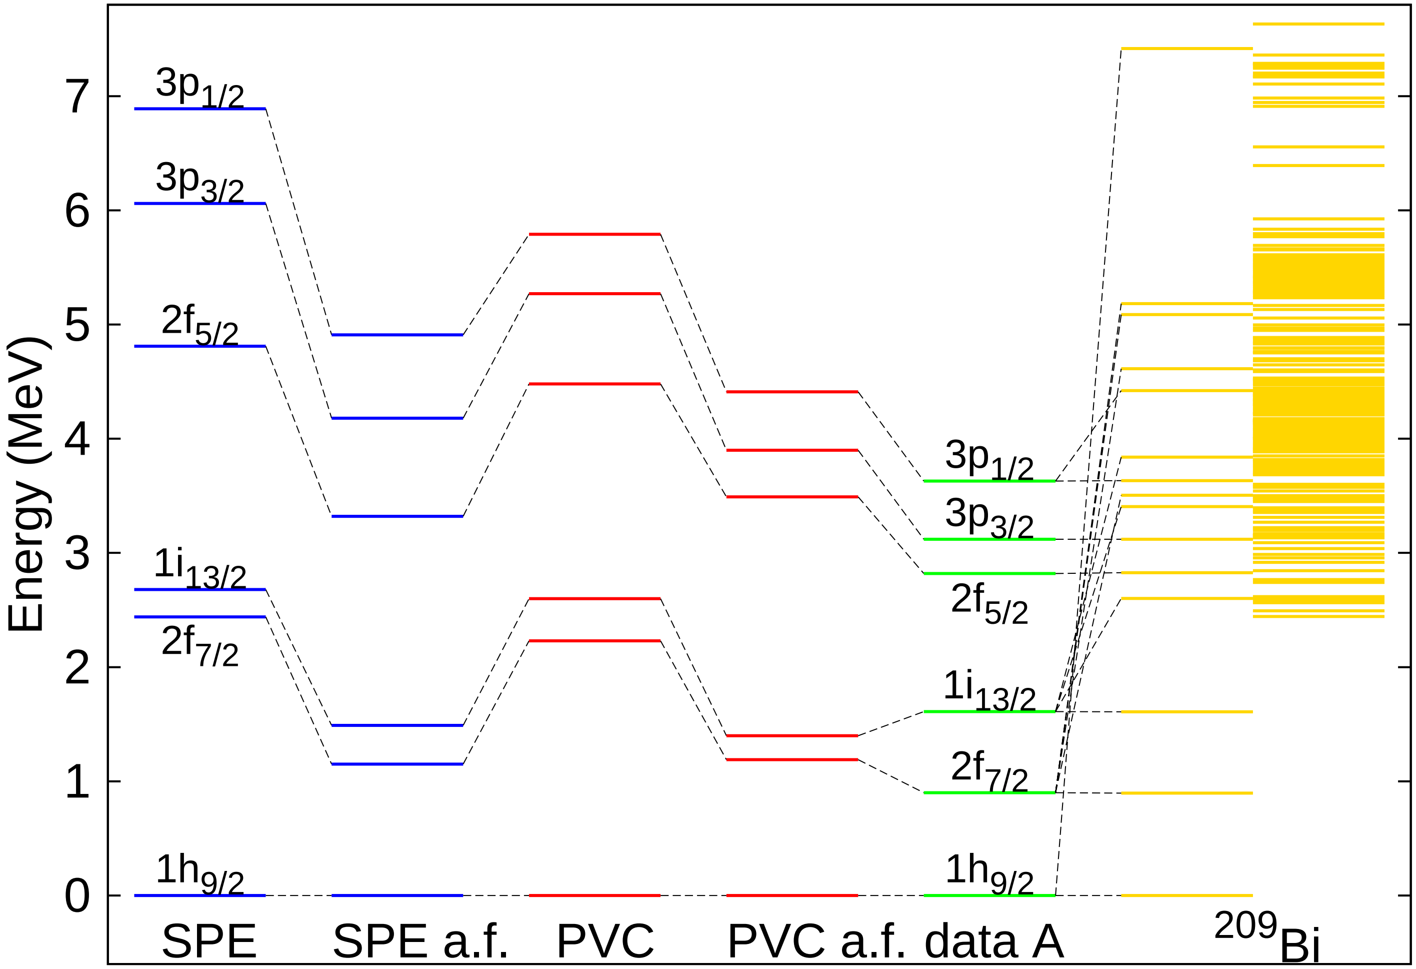


Figure 35: (Color online). Similar to Fig. 12, but for $^{209}$Bi.
